# Supplementary material for: Is ADC(3) as Accurate as CC3 for Valence and Rydberg Transition Energies?
Source: arXiv:1912.04806 source file (2019-12-13)
Supplement: Supplementary file 1 [file ADC-SI.pdf]

# Is ADC(3) as accurate as CC3 for valence and Rydberg transition energies? Supporting Information

Pierre-François Loos*,† and Denis Jacquemin*,‡

†*Laboratoire de Chimie et Physique Quantiques, Université de Toulouse, CNRS, UPS, France*

‡*Laboratoire CEISAM - UMR CNRS 6230, Université de Nantes, 2 Rue de la Houssinière, BP 92208, 44322 Nantes Cedex 3, France*

E-mail: loos@irsamc.ups-tlse.fr; Denis.Jacquemin@univ-nantes.fr

# Vertical energies

Below is a list of vertical transition energies obtained for a set of compounds described elsewhere.[1,2] These transition energies, obtained on CC3/*aug*-cc-pVTZ geometries, have been computed with the *aug*-cc-pVTZ basis set and within the frozen-core approximation. Note that the CC2, ADC(2) and CC3 data are already available in these previous works, and are reproduced below for the sake of completeness. To identify the ES with the different approaches considered here, we used the usual strategies, *i.e.*, relative energies, spatial and spin symmetries, symmetries and weights of the underlying molecular orbitals, and oscillator strengths. This allows unambiguous assignments for the vast majority of the states. There are however some state/method combinations for which strong mixing between ES of the same symmetry makes such assignments difficult. These challenging cases are nonetheless statistically irrelevant.

**Table S1: Comparisons between the TBE (see Refs. 1 and 2 for details and geometries) and the vertical excitation energies obtained with CC2, CC3, ADC(2), and ADC(3). All the values have been obtained with the *aug*-cc-pVTZ basis set and within the frozen-core approximation. We have removed from this training set all excited states with a dominant double excitation character. F, R and V stand for fluorescence, Rydberg and valence states, respectively.**

| Compound | State | TBE | CC2 | CC3 | ADC(2) | ADC(3) |
|---|---|---|---|---|---|---|
| Acetaldehyde | $^1A''(\text{V}; n \rightarrow \pi^\star)$ | 4.31 | 4.41 | 4.31 | 4.24 | 4.29 |
| | $^3A''(\text{V}; n \rightarrow \pi^\star)$ | 3.97 | 3.98 | 3.95 | 3.83 | 3.89 |
| Acetone | $^1A_2(\text{V}; n \rightarrow \pi^\star)$ | 4.47 | 4.55 | 4.48 | 4.37 | 4.50 |
| | $^1B_2(\text{R}; n \rightarrow 3s)$ | 6.46 | 5.91 | 6.43 | 5.87 | 6.91 |
| | $^1A_2(\text{R}; n \rightarrow 3p)$ | 7.47 | 6.84 | 7.45 | 6.81 | 7.90 |
| | $^1A_1(\text{R}; n \rightarrow 3p)$ | 7.51 | 6.89 | 7.48 | 6.85 | 7.92 |
| | $^1B_2(\text{R}; n \rightarrow 3p)$ | 7.62 | 7.02 | 7.59 | 6.99 | 8.01 |
| | $^3A_2(\text{V}; n \rightarrow \pi^\star)$ | 4.13 | 4.16 | 4.15 | 4.00 | 4.12 |
| | $^3A_1(\text{V}; \pi \rightarrow \pi^\star)$ | 6.25 | 6.50 | 6.28 | 6.37 | 6.01 |
| Acetylene | $^1\Sigma_u^-(\text{V}; \pi \rightarrow \pi^\star)$ | 7.10 | 7.26 | 7.09 | 7.24 | 6.72 |
| | $^1\Delta_u(\text{V}; \pi \rightarrow \pi^\star)$ | 7.44 | 7.59 | 7.42 | 7.56 | 7.06 |
| | $^3\Sigma_u^+(\text{V}; \pi \rightarrow \pi^\star)$ | 5.53 | 5.76 | 5.50 | 5.75 | 5.24 |
| | $^3\Delta_u(\text{V}; \pi \rightarrow \pi^\star)$ | 6.40 | 6.60 | 6.40 | 6.57 | 6.06 |
| | $^3\Sigma_u^-(\text{V}; \pi \rightarrow \pi^\star)$ | 7.08 | 7.29 | 7.07 | 7.27 | 6.72 |
| | $^1A_u[\text{F}](\text{V}; \pi \rightarrow \pi^\star)$ | 3.64 | 3.94 | 3.64 | 3.78 | 2.85 |
| | $^1A_2[\text{F}](\text{V}; \pi \rightarrow \pi^\star)$ | 3.85 | 4.11 | 3.84 | 3.99 | 3.08 |
| Acrolein | $^1A''(\text{V}; n \rightarrow \pi^\star)$ | 3.78 | 3.85 | 3.74 | 3.68 | 3.76 |
| | $^1A'(\text{V}; \pi \rightarrow \pi^\star)$ | 6.69 | 6.80 | 6.65 | 6.74 | 6.51 |

Continued on next page

| Compound | State | TBE | CC2 | CC3 | ADC(2) | ADC(3) |
| --- | --- | --- | --- | --- | --- | --- |
| | $^1A'(\mathrm{R}; n \to 3s)$ | 7.08 | 6.40 | 7.07 | 6.35 | 7.57 |
| | $^3A''(\mathrm{V}; n \to \pi^\star)$ | 3.51 | 3.49 | 3.46 | 3.33 | 3.45 |
| | $^3A'(\mathrm{V}; \pi \to \pi^\star)$ | 3.94 | 4.06 | 3.94 | 4.05 | 3.66 |
| | $^3A'(\mathrm{V}; \pi \to \pi^\star)$ | 6.18 | 6.37 | 6.19 | 6.31 | 5.86 |
| Ammonia | $^1A_2(\mathrm{R}; n \to 3s)$ | 6.59 | 6.39 | 6.57 | 6.40 | 6.63 |
| | $^1E(\mathrm{R}; n \to 3p)$ | 8.16 | 7.85 | 8.15 | 7.87 | 8.21 |
| | $^1A_1(\mathrm{R}; n \to 3p)$ | 9.33 | 9.05 | 9.32 | 9.05 | 9.38 |
| | $^1A_2(\mathrm{R}; n \to 4s)$ | 9.96 | 9.65 | 9.95 | 9.67 | 10.00 |
| | $^3A_2(\mathrm{R}; n \to 3s)$ | 6.31 | 6.14 | 6.29 | 6.16 | 6.31 |
| Carbon monoxyde | $^1\Pi(\mathrm{V}; n \to \pi^\star)$ | 8.49 | 8.64 | 8.49 | 8.69 | 8.24 |
| | $^1\Sigma^-(\mathrm{V}; \pi \to \pi^\star)$ | 9.92 | 10.30 | 9.99 | 10.03 | 9.73 |
| | $^1\Delta(\mathrm{V}; \pi \to \pi^\star)$ | 10.06 | 10.60 | 10.12 | 10.30 | 9.82 |
| | $^1\Sigma^+(\mathrm{R})$ | 10.95 | 11.11 | 10.94 | 11.32 | 10.79 |
| | $^1\Sigma^+(\mathrm{R})$ | 11.52 | 11.63 | 11.49 | 11.83 | 11.33 |
| | $^1\Pi(\mathrm{R})$ | 11.72 | 11.83 | 11.69 | 12.03 | 11.56 |
| | $^3\Pi(\mathrm{V}; n \to \pi^\star)$ | 6.28 | 6.42 | 6.30 | 6.45 | 5.97 |
| | $^3\Sigma^+(\mathrm{V}; \pi \to \pi^\star)$ | 8.45 | 8.72 | 8.45 | 8.54 | 8.21 |
| | $^3\Delta(\mathrm{V}; \pi \to \pi^\star)$ | 9.27 | 9.56 | 9.30 | 9.33 | 9.03 |
| | $^3\Sigma^-(\mathrm{V}; \pi \to \pi^\star)$ | 9.80 | 10.27 | 9.82 | 10.01 | 9.53 |
| | $^3\Sigma^+(\mathrm{R})$ | 10.47 | 10.60 | 10.45 | 10.83 | 10.29 |
| Benzene | $^1B_{2u}(\mathrm{V}; \pi \to \pi^\star)$ | 5.06 | 5.26 | 5.09 | 5.27 | 5.01 |
| | $^1B_{1u}(\mathrm{V}; \pi \to \pi^\star)$ | 6.45 | 6.48 | 6.44 | 6.45 | 6.24 |
| | $^1E_{1g}(\mathrm{R}; \pi \to 3s)$ | 6.52 | 6.47 | 6.52 | 6.52 | 6.38 |
| | $^1A_{2u}(\mathrm{R}; \pi \to 3p)$ | 7.08 | 7.00 | 7.08 | 7.06 | 6.92 |
| | $^1E_{2u}(\mathrm{R}; \pi \to 3p)$ | 7.15 | 7.06 | 7.15 | 7.12 | 7.00 |
| | $^3B_{1u}(\mathrm{V}; \pi \to \pi^\star)$ | 4.16 | 4.37 | 4.18 | 4.37 | 3.94 |
| | $^3E_{1u}(\mathrm{V}; \pi \to \pi^\star)$ | 4.85 | 5.08 | 4.86 | 5.07 | 4.60 |
| | $^3B_{2u}(\mathrm{V}; \pi \to \pi^\star)$ | 5.81 | 5.89 | 5.81 | 5.87 | 5.51 |
| Butadiene | $^1B_u(\mathrm{V}; \pi \to \pi^\star)$ | 6.22 | 6.16 | 6.22 | 6.12 | 6.02 |
| | $^1B_g(\mathrm{R}; \pi \to 3s)$ | 6.33 | 6.26 | 6.33 | 6.31 | 6.12 |
| | $^1A_g(\mathrm{V}; \pi \to \pi^\star)$ | 6.50 | 7.09 | 6.67 | 7.14 | 5.86 |
| | $^1A_u(\mathrm{R}; \pi \to 3p)$ | 6.64 | 6.57 | 6.64 | 6.63 | 6.44 |
| | $^1A_u(\mathrm{R}; \pi \to 3p)$ | 6.80 | 6.70 | 6.80 | 6.76 | 6.59 |
| | $^1B_u(\mathrm{R}; \pi \to 3p)$ | 7.68 | 7.63 | 7.68 | 7.48 | 7.46 |
| | $^3B_u(\mathrm{V}; \pi \to \pi^\star)$ | 3.36 | 3.45 | 3.36 | 3.46 | 3.09 |
| | $^3A_g(\mathrm{V}; \pi \to \pi^\star)$ | 5.20 | 5.30 | 5.20 | 5.27 | 4.94 |
| | $^3B_g(\mathrm{R}; \pi \to 3s)$ | 6.29 | 6.21 | 6.28 | 6.27 | 6.06 |
| Cyanoacetylene | $^1\Sigma^-(\mathrm{V}; \pi \to \pi^\star)$ | 5.80 | 6.03 | 5.80 | 5.99 | 5.37 |
| | $^1\Delta(\mathrm{V}; \pi \to \pi^\star)$ | 6.07 | 6.30 | 6.08 | 6.25 | 5.64 |
| | $^3\Sigma^+(\mathrm{V}; \pi \to \pi^\star)$ | 4.44 | 4.80 | 4.45 | 4.77 | 4.11 |
| | $^3\Delta(\mathrm{V}; \pi \to \pi^\star)$ | 5.21 | 5.50 | 5.22 | 5.46 | 4.80 |
| | $^1A''[\mathrm{F}](\mathrm{V}; \pi \to \pi^\star)$ | 3.54 | 3.79 | 3.54 | 3.73 | 2.78 |
| Cyanoformaldehyde | $^1A''(\mathrm{V}; n \to \pi^\star)$ | 3.81 | 3.97 | 3.83 | 3.83 | 3.77 |
| | $^1A''(\mathrm{V}; \pi \to \pi^\star)$ | 6.46 | 6.74 | 6.42 | 6.73 | 6.07 |
| | $^3A''(\mathrm{V}; n \to \pi^\star)$ | 3.44 | 3.51 | 3.46 | 3.37 | 3.38 |
| | $^3A'(\mathrm{V}; \pi \to \pi^\star)$ | 5.01 | 5.34 | 5.01 | 5.27 | 4.63 |
| Cyanogen | $^1\Sigma_u^-(\mathrm{V}; \pi \to \pi^\star)$ | 6.39 | 6.72 | 6.39 | 6.67 | 5.88 |
| | $^1\Delta_u(\mathrm{V}; \pi \to \pi^\star)$ | 6.66 | 7.02 | 6.66 | 6.95 | 6.16 |

Continued on next page

| Compound | State | TBE | CC2 | CC3 | ADC(2) | ADC(3) |
|---|---|---|---|---|---|---|
| | $^3\Sigma_u^+$(V; $\pi \rightarrow \pi^\star$) | 4.91 | 5.35 | 4.90 | 5.31 | 4.49 |
| | $^1\Sigma_u^-$[F](V; $\pi \rightarrow \pi^\star$) | 5.05 | 5.48 | 5.06 | 5.39 | 4.32 |
| Cyclopentadiene | $^1B_2$(V; $\pi \rightarrow \pi^\star$) | 5.56 | 5.52 | 5.54 | 5.49 | 5.35 |
| | $^1A_2$(R; $\pi \rightarrow 3s$) | 5.78 | 5.66 | 5.77 | 5.71 | 5.63 |
| | $^1B_1$(R; $\pi \rightarrow 3p$) | 6.41 | 6.26 | 6.40 | 6.31 | 6.25 |
| | $^1A_2$(R; $\pi \rightarrow 3p$) | 6.46 | 6.30 | 6.45 | 6.35 | 6.30 |
| | $^1B_2$(R; $\pi \rightarrow 3p$) | 6.56 | 6.42 | 6.56 | 6.48 | 6.41 |
| | $^3B_2$(V; $\pi \rightarrow \pi^\star$) | 3.31 | 3.42 | 3.32 | 3.42 | 3.05 |
| | $^3A_1$(V; $\pi \rightarrow \pi^\star$) | 5.11 | 5.36 | 5.12 | 5.23 | 4.86 |
| | $^3A_2$(R; $\pi \rightarrow 3s$) | 5.73 | 5.62 | 5.73 | 5.67 | 5.57 |
| | $^3B_1$(R; $\pi \rightarrow 3p$) | 6.36 | 6.22 | 6.36 | 6.27 | 6.20 |
| Cyclopropene | $^1B_1$(V; $\sigma \rightarrow \pi^\star$) | 6.68 | 6.73 | 6.68 | 6.75 | 6.56 |
| | $^1B_2$(V; $\pi \rightarrow \pi^\star$) | 6.79 | 6.78 | 6.73 | 6.86 | 6.56 |
| | $^3B_2$(V; $\pi \rightarrow \pi^\star$) | 4.38 | 4.46 | 4.34 | 4.45 | 4.09 |
| | $^3B_1$(V; $\sigma \rightarrow \pi^\star$) | 6.45 | 6.44 | 6.40 | 6.45 | 6.26 |
| Cyclopropenone | $^1B_1$(V; $n \rightarrow \pi^\star$) | 4.26 | 4.01 | 4.21 | 3.88 | 4.66 |
| | $^1A_2$(V; $n \rightarrow \pi^\star$) | 5.55 | 5.65 | 5.57 | 5.47 | 5.61 |
| | $^1B_2$(R; $n \rightarrow 3s$) | 6.34 | 5.84 | 6.32 | 5.79 | 6.64 |
| | $^1B_2$(V; $\pi \rightarrow \pi^\star$) | 6.54 | 6.46 | 6.54 | 6.33 | 6.83 |
| | $^1B_2$(R; $n \rightarrow 3p$) | 6.98 | 6.56 | 6.96 | 6.43 | 7.33 |
| | $^1A_1$(R; $n \rightarrow 3p$) | 7.02 | 6.47 | 7.00 | 6.41 | 7.36 |
| | $^1A_1$(V; $\pi \rightarrow \pi^\star$) | 8.28 | 8.28 | 8.28 | 8.10 | 8.17 |
| | $^3B_1$(V; $n \rightarrow \pi^\star$) | 3.93 | 3.73 | 3.91 | 3.62 | 4.28 |
| | $^3B_2$(V; $\pi \rightarrow \pi^\star$) | 4.88 | 4.99 | 4.89 | 4.90 | 4.80 |
| | $^3A_2$(V; $n \rightarrow \pi^\star$) | 5.35 | 5.45 | 5.37 | 5.28 | 5.36 |
| | $^3A_1$(V; $\pi \rightarrow \pi^\star$) | 6.79 | 6.42 | 6.83 | 6.84 | 6.63 |
| Cyclopropenethione | $^1A_2$(V; $n \rightarrow \pi^\star$) | 3.41 | 3.53 | 3.43 | 3.38 | 3.46 |
| | $^1B_1$(V; $n \rightarrow \pi^\star$) | 3.45 | 3.50 | 3.43 | 3.37 | 3.82 |
| | $^1B_2$(V; $\pi \rightarrow \pi^\star$) | 4.60 | 4.91 | 4.64 | 4.72 | 4.72 |
| | $^1B_2$(R; $n \rightarrow 3s$) | 5.34 | 5.22 | 5.34 | 5.17 | 5.41 |
| | $^1A_1$(V; $\pi \rightarrow \pi^\star$) | 5.46 | 5.59 | 5.49 | 5.36 | 5.36 |
| | $^1B_2$(R; $n \rightarrow 3p$) | 5.92 | 5.82 | 5.93 | 5.77 | 6.02 |
| | $^3A_2$(V; $n \rightarrow \pi^\star$) | 3.28 | 3.37 | 3.30 | 3.23 | 3.30 |
| | $^3B_1$(V; $n \rightarrow \pi^\star$) | 3.32 | 3.38 | 3.31 | 3.26 | 3.65 |
| | $^3B_2$(V; $\pi \rightarrow \pi^\star$) | 4.01 | 4.24 | 4.02 | 4.12 | 3.96 |
| | $^3A_1$(V; $\pi \rightarrow \pi^\star$) | 4.01 | 4.16 | 4.03 | 4.04 | 3.83 |
| Diacetylene | $^1\Sigma_u^-$(V; $\pi \rightarrow \pi^\star$) | 5.33 | 5.51 | 5.34 | 5.49 | 4.95 |
| | $^1\Delta_u$(V; $\pi \rightarrow \pi^\star$) | 5.61 | 5.76 | 5.61 | 5.72 | 5.22 |
| | $^3\Sigma_u^+$(V; $\pi \rightarrow \pi^\star$) | 4.10 | 4.39 | 4.08 | 4.37 | 3.79 |
| | $^3\Delta_u$(V; $\pi \rightarrow \pi^\star$) | 4.78 | 5.03 | 4.80 | 5.01 | 4.43 |
| Diazomethane | $^1A_2$(V; $\pi \rightarrow \pi^\star$) | 3.14 | 3.37 | 3.07 | 3.34 | 2.74 |
| | $^1B_1$(R; $\pi \rightarrow 3s$) | 5.54 | 5.53 | 5.45 | 5.63 | 5.23 |
| | $^1A_1$(V; $\pi \rightarrow \pi^\star$) | 5.90 | 6.00 | 5.84 | 5.97 | 5.48 |
| | $^3A_2$(V; $\pi \rightarrow \pi^\star$) | 2.79 | 3.08 | 2.83 | 3.01 | 2.44 |
| | $^3A_1$(V; $\pi \rightarrow \pi^\star$) | 4.05 | 4.25 | 4.03 | 4.20 | 3.64 |
| | $^3B_1$(R; $\pi \rightarrow 3s$) | 5.35 | 5.53 | 5.31 | 5.50 | 5.08 |
| | $^3A_1$(R; $\pi \rightarrow 3p$) | 6.82 | 7.04 | 6.80 | 7.09 | 6.36 |
| | $^1A''$[F](V; $\pi \rightarrow \pi^\star$) | 0.71 | 0.90 | 0.68 | 0.81 | 0.24 |

Continued on next page

| Compound | State | TBE | CC2 | CC3 | ADC(2) | ADC(3) |
|---|---|---|---|---|---|---|
| Dinitrogen | $^1\Pi_g(\text{V}; n \rightarrow \pi^\star)$ | 9.34 | 9.44 | 9.34 | 9.48 | 9.16 |
| | $^1\Sigma_u^-(\text{V}; \pi \rightarrow \pi^\star)$ | 9.88 | 10.32 | 9.88 | 10.26 | 9.33 |
| | $^1\Delta_u(\text{V}; \pi \rightarrow \pi^\star)$ | 10.29 | 10.86 | 10.29 | 10.79 | 9.74 |
| | $^1\Sigma_g^+(\text{R})$ | 12.98 | 12.83 | 13.01 | 12.99 | 13.01 |
| | $^1\Pi_u(\text{R})$ | 13.03 | 13.15 | 13.22 | 13.32 | 12.98 |
| | $^1\Sigma_u^+(\text{R})$ | 13.09 | 12.89 | 13.12 | 13.07 | 13.09 |
| | $^1\Pi_u(\text{R})$ | 13.46 | 13.96 | 13.49 | 14.00 | 13.40 |
| | $^3\Sigma_u^+(\text{V}; \pi \rightarrow \pi^\star)$ | 7.70 | 8.19 | 7.68 | 8.15 | 7.25 |
| | $^3\Pi_g(\text{V}; n \rightarrow \pi^\star)$ | 8.01 | 8.19 | 8.04 | 8.20 | 7.77 |
| | $^3\Delta_u(\text{V}; \pi \rightarrow \pi^\star)$ | 8.87 | 9.30 | 8.87 | 9.25 | 8.36 |
| | $^3\Sigma_u^-(\text{V}; \pi \rightarrow \pi^\star)$ | 9.66 | 10.29 | 9.68 | 10.23 | 9.14 |
| Ethylene | $^1B_{3u}(\text{R}; \pi \rightarrow 3s)$ | 7.39 | 7.29 | 7.35 | 7.34 | 7.17 |
| | $^1B_{1u}(\text{V}; \pi \rightarrow \pi^\star)$ | 7.93 | 7.92 | 7.91 | 7.91 | 7.69 |
| | $^1B_{1g}(\text{R}; \pi \rightarrow 3p)$ | 8.08 | 7.95 | 8.03 | 7.99 | 7.84 |
| | $^3B_{1u}(\text{V}; \pi \rightarrow \pi^\star)$ | 4.54 | 4.59 | 4.53 | 4.59 | 4.28 |
| | $^3B_{3u}(\text{R}; \pi \rightarrow 3s)$ | 7.23 | 7.19 | 7.24 | 7.23 | 7.05 |
| | $^3B_{1g}(\text{R}; \pi \rightarrow 3p)$ | 7.98 | 7.91 | 7.98 | 7.95 | 7.80 |
| Formaldehyde | $^1A_2(\text{V}; n \rightarrow \pi^\star)$ | 3.98 | 4.07 | 3.97 | 3.92 | 3.90 |
| | $^1B_2(\text{R}; n \rightarrow 3s)$ | 7.23 | 6.56 | 7.18 | 6.50 | 7.62 |
| | $^1B_2(\text{R}; n \rightarrow 3p)$ | 8.13 | 7.57 | 8.07 | 7.53 | 8.45 |
| | $^1A_1(\text{R}; n \rightarrow 3p)$ | 8.23 | 7.52 | 8.18 | 7.47 | 8.61 |
| | $^1A_2(\text{R}; n \rightarrow 3p)$ | 8.67 | 8.04 | 8.64 | 7.99 | 9.02 |
| | $^1B_1(\text{V}; \sigma \rightarrow \pi^\star)$ | 9.22 | 9.32 | 9.19 | 9.17 | 9.17 |
| | $^1A_1(\text{V}; \pi \rightarrow \pi^\star)$ | 9.43 | 9.54 | 9.48 | 9.46 | 9.05 |
| | $^3A_2(\text{V}; n \rightarrow \pi^\star)$ | 3.58 | 3.59 | 3.57 | 3.46 | 3.48 |
| | $^3A_1(\text{V}; \pi \rightarrow \pi^\star)$ | 6.06 | 6.30 | 6.05 | 6.20 | 5.71 |
| | $^3B_2(\text{R}; n \rightarrow 3s)$ | 7.06 | 6.44 | 7.03 | 6.39 | 7.44 |
| | $^3B_2(\text{R}; n \rightarrow 3p)$ | 7.94 | 7.45 | 7.92 | 7.41 | 8.23 |
| | $^3A_1(\text{R}; n \rightarrow 3p)$ | 8.10 | 7.44 | 8.08 | 7.40 | 8.46 |
| | $^3B_1(\text{R}; n \rightarrow 3d)$ | 8.42 | 8.52 | 8.41 | 8.39 | 8.32 |
| | $^1A$"[F]$(\text{V}; n \rightarrow \pi^\star)$ | 2.80 | 2.97 | 2.84 | 2.71 | 2.77 |
| Formamide | $^1A''(\text{V}; n \rightarrow \pi^\star)$ | 5.65 | 5.69 | 5.66 | 5.45 | 5.75 |
| | $^3A''(\text{V}; n \rightarrow \pi^\star)$ | 5.38 | 5.36 | 5.38 | 5.15 | 5.42 |
| | $^3A'(\text{V}; \pi \rightarrow \pi^\star)$ | 5.81 | 5.99 | 5.82 | 5.88 | 5.63 |
| Furan | $^1A_2(\text{R}; \pi \rightarrow 3s)$ | 6.09 | 6.06 | 6.08 | 6.12 | 5.95 |
| | $^1B_2(\text{V}; \pi \rightarrow \pi^\star)$ | 6.37 | 6.45 | 6.34 | 6.47 | 6.15 |
| | $^1A_1(\text{V}; \pi \rightarrow \pi^\star)$ | 6.56 | 6.77 | 6.58 | 6.76 | 6.48 |
| | $^1B_1(\text{R}; \pi \rightarrow 3p)$ | 6.64 | 6.59 | 6.63 | 6.64 | 6.49 |
| | $^1A_2(\text{R}; \pi \rightarrow 3p)$ | 6.81 | 6.75 | 6.80 | 6.82 | 6.67 |
| | $^1B_2(\text{R}; \pi \rightarrow 3p)$ | 7.24 | 7.25 | 7.23 | 7.29 | 7.09 |
| | $^3B_2(\text{V}; \pi \rightarrow \pi^\star)$ | 4.20 | 4.43 | 4.22 | 4.41 | 3.91 |
| | $^3A_1(\text{V}; \pi \rightarrow \pi^\star)$ | 5.46 | 5.66 | 5.48 | 5.59 | 5.23 |
| | $^3A_2(\text{R}; \pi \rightarrow 3s)$ | 6.02 | 6.01 | 6.02 | 6.08 | 5.89 |
| | $^3B_1(\text{R}; \pi \rightarrow 3p)$ | 6.59 | 6.55 | 6.59 | 6.61 | 6.45 |
| Glyoxal | $^1A_u(\text{V}; n \rightarrow \pi^\star)$ | 2.88 | 2.91 | 2.88 | 2.83 | 2.83 |
| | $^1B_g(\text{V}; n \rightarrow \pi^\star)$ | 4.24 | 4.44 | 4.27 | 4.27 | 4.23 |
| | $^1B_g(\text{V}; n \rightarrow \pi^\star)$ | 6.57 | 6.51 | 6.58 | 6.50 | 6.80 |
| | $^1B_u(\text{R}; n \rightarrow 3p)$ | 7.71 | 7.16 | 7.67 | 7.18 | 7.86 |

Continued on next page

| Compound | State | TBE | CC2 | CC3 | ADC(2) | ADC(3) |
|---|---|---|---|---|---|---|
| | $^3A_u$(V; $n \rightarrow \pi^\star$) | 2.49 | 2.47 | 2.49 | 2.39 | 2.40 |
| | $^3B_g$(V; $n \rightarrow \pi^\star$) | 3.89 | 3.96 | 3.90 | 3.82 | 3.85 |
| | $^3B_u$(V; $\pi \rightarrow \pi^\star$) | 5.15 | 5.42 | 5.17 | 5.33 | 4.83 |
| | $^3A_g$(V; $\pi \rightarrow \pi^\star$) | 6.30 | 6.56 | 6.30 | 6.45 | 5.93 |
| Hydrogen chloride | $^1\Pi$(CT) | 7.84 | 7.96 | 7.84 | 7.97 | 7.79 |
| Hydrogen sulfide | $^1A_2$(R; $n \rightarrow 4p$) | 6.18 | 6.35 | 6.19 | 6.37 | 6.05 |
| | $^1B_1$(R; $n \rightarrow 4s$) | 6.24 | 6.30 | 6.24 | 6.34 | 6.18 |
| | $^3A_2$(R; $n \rightarrow 4p$) | 5.81 | 5.91 | 5.82 | 5.91 | 5.67 |
| | $^3B_1$(R; $n \rightarrow 4s$) | 5.88 | 5.94 | 5.88 | 5.96 | 5.81 |
| Imidazole | $^1A''$(R; $\pi \rightarrow 3s$) | 5.71 | 5.69 | 5.71 | 5.75 | 5.61 |
| | $^1A'$(V; $\pi \rightarrow \pi^\star$) | 6.41 | 6.51 | 6.41 | 6.50 | 6.31 |
| | $^1A''$(V; $n \rightarrow \pi^\star$) | 6.50 | 6.47 | 6.50 | 6.51 | 6.39 |
| | $^3A'$(V; $\pi \rightarrow \pi^\star$) | 4.73 | 4.94 | 4.75 | 4.92 | 4.47 |
| | $^3A''$(R; $\pi \rightarrow 3s$) | 5.66 | 5.66 | 5.67 | 5.72 | 5.57 |
| | $^3A'$(V; $\pi \rightarrow \pi^\star$) | 5.74 | 5.94 | 5.74 | 5.93 | 5.49 |
| | $^3A''$(V; $n \rightarrow \pi^\star$) | 6.31 | 6.36 | 6.33 | 6.31 | 6.26 |
| Isobutene | $^1B_1$(R; $\pi \rightarrow 3s$) | 6.46 | 6.37 | 6.45 | 6.43 | 6.33 |
| | $^1A_1$(R; $\pi \rightarrow 3p$) | 7.01 | 6.95 | 7.00 | 6.97 | 6.82 |
| | $^3A_1$(V; ($\pi \rightarrow \pi^\star$) | 4.53 | 4.62 | 4.53 | 4.62 | 4.30 |
| Ketene | $^1A_2$(V; $\pi \rightarrow \pi^\star$) | 3.86 | 4.17 | 3.88 | 4.11 | 3.67 |
| | $^1B_1$(R; $n \rightarrow 3s$) | 6.01 | 5.94 | 5.96 | 6.03 | 5.87 |
| | $^1A_2$(R; $\pi \rightarrow 3p$) | 7.18 | 7.09 | 7.16 | 7.18 | 7.07 |
| | $^3A_2$(V; $n \rightarrow \pi^\star$) | 3.77 | 3.98 | 3.78 | 3.92 | 3.56 |
| | $^3A_1$(V; $\pi \rightarrow \pi^\star$) | 5.61 | 5.72 | 5.61 | 5.67 | 5.39 |
| | $^3B_1$(R; $n \rightarrow 3s$) | 5.79 | 5.77 | 5.76 | 5.85 | 5.67 |
| | $^3A_2$(R; $\pi \rightarrow 3p$) | 7.12 | 7.06 | 7.12 | 7.15 | 7.03 |
| | $^1A$"[F](V; $\pi \rightarrow \pi^\star$) | 1.00 | 1.26 | 1.00 | 1.19 | 0.67 |
| Methanimine | $^1A$"(V; $n \rightarrow \pi^\star$) | 5.23 | 5.32 | 5.20 | 5.29 | 5.05 |
| | $^3A$"(V; $n \rightarrow \pi^\star$) | 4.65 | 4.65 | 4.61 | 4.61 | 4.44 |
| Methylenecyclopropene | $^1B_2$(V; $\pi \rightarrow \pi^\star$) | 4.28 | 4.51 | 4.31 | 4.46 | 4.18 |
| | $^1B_1$(R; $\pi \rightarrow 3s$) | 5.44 | 5.35 | 5.44 | 5.38 | 5.26 |
| | $^1A_2$(R; $\pi \rightarrow 3p$) | 5.96 | 5.85 | 5.95 | 5.87 | 5.78 |
| | $^3B_2$(V; $\pi \rightarrow \pi^\star$) | 3.49 | 3.64 | 3.50 | 3.61 | 3.30 |
| | $^3A_1$(V; $\pi \rightarrow \pi^\star$) | 4.74 | 4.81 | 4.74 | 4.80 | 4.51 |
| Nitrosomethane | $^1A''$(V; $n \rightarrow \pi^\star$) | 1.96 | 1.98 | 1.96 | 1.88 | 1.72 |
| | $^1A'$(R; $n \rightarrow 3s/3p$) | 6.40 | 5.84 | 6.31 | 5.86 | 6.48 |
| | $^3A''$(V; $n \rightarrow \pi^\star$) | 1.16 | 1.12 | 1.14 | 1.03 | 0.84 |
| | $^3A'$(V; $\pi \rightarrow \pi^\star$) | 5.60 | 5.74 | 5.51 | 5.75 | 5.04 |
| | $^1A''$[F](V; $n \rightarrow \pi^\star$) | 1.67 | 1.68 | 1.69 | 1.55 | 1.40 |
| Propynal | $^1A''$(V; $n \rightarrow \pi^\star$) | 3.80 | 3.96 | 3.82 | 3.78 | 3.81 |
| | $^1A''$(V; $\pi \rightarrow \pi^\star$) | 5.54 | 5.71 | 5.51 | 5.73 | 5.20 |
| | $^3A''$(V; $n \rightarrow \pi^\star$) | 3.47 | 3.53 | 3.49 | 3.38 | 3.45 |
| | $^3A'$(V; $\pi \rightarrow \pi^\star$) | 4.47 | 4.71 | 4.43 | 4.67 | 4.10 |
| Pyrazine | $^1B_{3u}$(V; $n \rightarrow \pi^\star$) | 4.15 | 4.14 | 4.14 | 4.17 | 4.13 |
| | $^1A_u$(V; $n \rightarrow \pi^\star$) | 4.98 | 4.86 | 4.97 | 4.88 | 5.21 |
| | $^1B_{2u}$(V; $\pi \rightarrow \pi^\star$) | 5.02 | 5.14 | 5.03 | 5.47 | 4.88 |
| | $^1B_{2g}$(V; $n \rightarrow \pi^\star$) | 5.71 | 5.86 | 5.71 | 5.87 | 5.67 |
| | $^1A_g$(R; $n \rightarrow 3s$) | 6.65 | 6.20 | 6.66 | 6.30 | 6.96 |

Continued on next page

| Compound | State | TBE | CC2 | CC3 | ADC(2) | ADC(3) |
|---|---|---|---|---|---|---|
| | $^1B_{1g}(\mathrm{V}; n \to \pi^\star)$ | 6.74 | 6.67 | 6.73 | 6.67 | 7.00 |
| | $^1B_{1u}(\mathrm{V}; \pi \to \pi^\star)$ | 6.88 | 6.89 | 6.86 | 6.88 | 6.66 |
| | $^1B_{1g}(\mathrm{R}; \pi \to 3s)$ | 7.21 | 7.21 | 7.20 | 7.27 | 7.18 |
| | $^1B_{2u}(\mathrm{R}; n \to 3p)$ | 7.24 | 6.74 | 7.25 | | |
| | $^1B_{1u}(\mathrm{R}; n \to 3p)$ | 7.44 | 7.03 | 7.45 | | |
| | $^3B_{3u}(\mathrm{V}; n \to \pi^\star)$ | 3.59 | 3.60 | 3.59 | 3.62 | 3.52 |
| | $^3B_{1u}(\mathrm{V}; \pi \to \pi^\star)$ | 4.35 | 4.60 | 4.39 | 4.57 | 4.05 |
| | $^3B_{2u}(\mathrm{V}; (\pi \to \pi^\star)$ | 4.39 | 4.57 | 4.40 | 4.59 | 4.10 |
| | $^3A_{u}(\mathrm{V}; n \to \pi^\star)$ | 4.93 | 4.82 | 4.93 | 4.84 | 5.15 |
| | $^3B_{2g}(\mathrm{V}; n \to \pi^\star)$ | 5.08 | 5.19 | 5.08 | | |
| | $^3B_{1u}(\mathrm{V}; \pi \to \pi^\star)$ | 5.28 | 5.59 | 5.29 | | |
| Pyridazine | $^1B_{1}(\mathrm{V}; n \to \pi^\star)$ | 3.83 | 3.78 | 3.83 | 3.79 | 3.86 |
| | $^1A_{2}(\mathrm{V}; n \to \pi^\star)$ | 4.37 | 4.26 | 4.37 | 4.27 | 4.60 |
| | $^1A_{1}(\mathrm{V}; \pi \to \pi^\star)$ | 5.26 | 5.43 | 5.29 | 5.44 | 5.18 |
| | $^1A_{2}(\mathrm{V}; n \to \pi^\star)$ | 5.72 | 5.79 | 5.74 | 5.81 | 5.74 |
| | $^1B_{2}(\mathrm{R}; n \to 3s)$ | 6.17 | 5.59 | 6.17 | 5.69 | 6.67 |
| | $^1B_{1}(\mathrm{V}; n \to \pi^\star)$ | 6.37 | 6.33 | 6.37 | 6.35 | 6.62 |
| | $^1B_{2}(\mathrm{V}; \pi \to \pi^\star)$ | 6.75 | 6.86 | 6.74 | 6.85 | |
| | $^3B_{1}(\mathrm{V}; n \to \pi^\star)$ | 3.19 | 3.18 | 3.19 | 3.19 | 3.12 |
| | $^3A_{2}(\mathrm{V}; n \to \pi^\star)$ | 4.11 | 4.01 | 4.11 | 4.02 | 4.22 |
| | $^3A_{1}(\mathrm{V}; \pi \to \pi^\star)$ | 4.82 | 5.07 | 4.83 | 5.06 | 4.46 |
| Pyridine | $^1B_{1}(\mathrm{V}; n \to \pi^\star)$ | 4.95 | 4.99 | 4.96 | 4.98 | 4.99 |
| | $^1B_{2}(\mathrm{V}; \pi \to \pi^\star)$ | 5.14 | 5.32 | 5.17 | 5.33 | 5.08 |
| | $^1A_{2}(\mathrm{V}; n \to \pi^\star)$ | 5.40 | 5.28 | 5.40 | 5.27 | 5.70 |
| | $^1A_{1}(\mathrm{V}; \pi \to \pi^\star)$ | 6.62 | 6.21 | 6.63 | 6.31 | 7.17 |
| | $^1A_{1}(\mathrm{R}; n \to 3s)$ | 6.76 | 6.68 | 6.76 | 6.65 | 6.39 |
| | $^1A_{2}(\mathrm{R}; \pi \to 3s)$ | 6.82 | 6.79 | 6.81 | 6.83 | 6.65 |
| | $^1B_{1}(\mathrm{R}; \pi \to 3p)$ | 7.39 | 7.34 | 7.38 | 7.38 | 7.21 |
| | $^1A_{1}(\mathrm{V}; \pi \to \pi^\star)$ | 7.39 | 7.45 | 7.39 | 7.48 | 7.27 |
| | $^3A_{1}(\mathrm{V}; \pi \to \pi^\star)$ | 4.30 | 4.53 | 4.33 | 4.53 | 4.06 |
| | $^3B_{1}(\mathrm{V}; n \to \pi^\star)$ | 4.46 | 4.48 | 4.46 | 4.47 | 4.43 |
| | $^3B_{2}(\mathrm{V}; \pi \to \pi^\star)$ | 4.79 | 4.98 | 4.79 | 4.98 | 4.49 |
| | $^3A_{1}(\mathrm{V}; \pi \to \pi^\star)$ | 5.04 | 5.29 | 5.05 | 5.28 | 4.75 |
| | $^3A_{2}(\mathrm{V}; n \to \pi^\star)$ | 5.36 | 5.24 | 5.35 | 5.23 | 5.62 |
| | $^3B_{2}(\mathrm{V}; \pi \to \pi^\star)$ | 6.24 | 6.39 | 6.25 | 6.35 | 5.98 |
| Pyrimidine | $^1B_{1}(\mathrm{V}; n \to \pi^\star)$ | 4.44 | 4.41 | 4.44 | 4.37 | 4.54 |
| | $^1A_{2}(\mathrm{V}; n \to \pi^\star)$ | 4.85 | 4.77 | 4.86 | 4.73 | 5.06 |
| | $^1B_{2}(\mathrm{V}; \pi \to \pi^\star)$ | 5.38 | 5.54 | 5.41 | 5.52 | 5.33 |
| | $^1A_{2}(\mathrm{V}; n \to \pi^\star)$ | 5.92 | 5.96 | 5.93 | 5.93 | 6.08 |
| | $^1B_{1}(\mathrm{V}; n \to \pi^\star)$ | 6.26 | 6.25 | 6.26 | 6.22 | 6.52 |
| | $^1B_{2}(\mathrm{R}; n \to 3s)$ | 6.70 | 6.20 | 6.72 | 6.25 | 7.11 |
| | $^1A_{1}(\mathrm{V}; \pi \to \pi^\star)$ | 6.88 | 6.84 | 6.87 | 6.83 | 6.52 |
| | $^3B_{1}(\mathrm{V}; n \to \pi^\star)$ | 4.09 | 4.07 | 4.10 | 4.05 | 4.12 |
| | $^3A_{2}(\mathrm{V}; n \to \pi^\star)$ | 4.66 | 4.60 | 4.66 | 4.58 | 4.73 |
| | $^3B_{2}(\mathrm{V}; \pi \to \pi^\star)$ | 4.96 | 5.17 | 4.96 | 5.14 | 4.63 |
| Pyrrole | $^1A_{2}(\mathrm{R}; \pi \to 3s)$ | 5.24 | 5.23 | 5.24 | 5.30 | 5.14 |
| | $^1B_{1}(\mathrm{R}; \pi \to 3p)$ | 6.00 | 5.91 | 5.98 | 5.94 | 5.89 |
| | $^1A_{2}(\mathrm{R}; \pi \to 3p)$ | 6.00 | 5.96 | 6.01 | 6.03 | 5.91 |

Continued on next page

| Compound | State | TBE | CC2 | CC3 | ADC(2) | ADC(3) |
|---|---|---|---|---|---|---|
| | $^1B_2$(V; $(\pi \rightarrow \pi^\star)$ | 6.26 | 6.30 | 6.25 | 6.35 | 6.11 |
| | $^1A_1$(V; $\pi \rightarrow \pi^\star$) | 6.30 | 6.47 | 6.32 | 6.47 | 6.29 |
| | $^1B_2$(R; $\pi \rightarrow 3p$) | 6.83 | 6.89 | 6.83 | 6.91 | 6.69 |
| | $^3B_2$(V; $\pi \rightarrow \pi^\star$) | 4.51 | 4.72 | 4.53 | 4.71 | 4.26 |
| | $^3A_2$(R; $\pi \rightarrow 3s$) | 5.21 | 5.20 | 5.21 | 5.27 | 5.11 |
| | $^3A_1$(V; $\pi \rightarrow \pi^\star$) | 5.45 | 5.66 | 5.46 | 5.62 | 5.23 |
| | $^3B_1$(R; $\pi \rightarrow 3p$) | 5.91 | 5.86 | 5.92 | 5.89 | 5.84 |
| Streptocyanine | $^1B_2$(V; $\pi \rightarrow \pi^\star$) | 7.13 | 7.20 | 7.13 | 7.00 | 7.16 |
| | $^3B_2$(V; $\pi \rightarrow \pi^\star$) | 5.47 | 5.60 | 5.48 | 5.55 | 5.33 |
| Tetrazine | $^1B_{3u}$(V; $n \rightarrow \pi^\star$) | 2.47 | 2.38 | 2.46 | 2.42 | 2.42 |
| | $^1A_u$(V; $n \rightarrow \pi^\star$) | 3.69 | 3.53 | 3.67 | 3.58 | 3.87 |
| | $^1B_{1g}$(V; $n \rightarrow \pi^\star$) | 4.93 | 5.02 | 4.91 | 5.04 | 4.97 |
| | $^1B_{2u}$(V; $\pi \rightarrow \pi^\star$) | 5.21 | 5.31 | 5.23 | 5.31 | 5.08 |
| | $^1B_{2g}$(V; $n \rightarrow \pi^\star$) | 5.45 | 5.64 | 5.46 | 5.68 | 5.13 |
| | $^1A_u$(V; $n \rightarrow \pi^\star$) | 5.53 | 5.56 | 5.52 | 5.59 | 5.49 |
| | $^1B_{2g}$(V; $n \rightarrow \pi^\star$) | 6.12 | 6.18 | 6.13 | 6.21 | 6.50 |
| | $^1B_{1g}$(V; $n \rightarrow \pi^\star$) | 6.91 | 6.95 | 6.92 | 6.97 | 6.59 |
| | $^3B_{3u}$(V; $n \rightarrow \pi^\star$) | 1.85 | 1.81 | 1.85 | 1.85 | 1.74 |
| | $^3A_u$(V; $n \rightarrow \pi^\star$) | 3.45 | 3.31 | 3.44 | 3.35 | 3.54 |
| | $^3B_{1g}$(V; $n \rightarrow \pi^\star$) | 4.20 | 4.27 | 4.20 | 4.27 | 4.06 |
| | $^3B_{2u}$(V; $\pi \rightarrow \pi^\star$) | 4.52 | 4.77 | 4.52 | 4.76 | 4.06 |
| | $^3B_{2g}$(V; $n \rightarrow \pi^\star$) | 5.04 | 5.15 | 5.05 | 5.16 | 4.86 |
| | $^3A_u$(V; $n \rightarrow \pi^\star$) | 5.11 | 5.13 | 5.11 | 5.16 | 5.07 |
| | $^3B_{1u}$(V; $\pi \rightarrow \pi^\star$) | 5.42 | 5.70 | 5.42 | 5.67 | 5.06 |
| Thioacetone | $^1A_2$(V; $n \rightarrow \pi^\star$) | 2.53 | 2.63 | 2.55 | 2.47 | 2.50 |
| | $^1B_2$(R; $n \rightarrow 4s$) | 5.56 | 5.50 | 5.55 | 5.47 | 5.65 |
| | $^1A_1$(V; $\pi \rightarrow \pi^\star$) | 5.88 | 6.09 | 5.90 | 5.87 | 5.53 |
| | $^1B_2$(R; $n \rightarrow 4p$) | 6.51 | 6.53 | 6.51 | 6.43 | 6.53 |
| | $^1A_1$(R; $n \rightarrow 4p$) | 6.61 | 6.44 | 6.61 | 6.48 | 6.64 |
| | $^3A_2$(V; $n \rightarrow \pi^\star$) | 2.33 | 2.33 | 2.34 | 2.20 | 2.26 |
| | $^3A_1$(V; $\pi \rightarrow \pi^\star$) | 3.45 | 3.59 | 3.46 | 3.52 | 3.17 |
| Thioformaldehyde | $^1A_2$(V; $n \rightarrow \pi^\star$) | 2.22 | 2.34 | 2.23 | 2.24 | 2.05 |
| | $^1B_2$(R; $n \rightarrow 4s$) | 5.96 | 5.82 | 5.91 | 5.80 | 5.94 |
| | $^1A_1$(V; $\pi \rightarrow \pi^\star$) | 6.38 | 6.71 | 6.48 | 6.57 | 5.98 |
| | $^3A_2$(V; $n \rightarrow \pi^\star$) | 1.94 | 1.94 | 1.94 | 1.86 | 1.77 |
| | $^3A_1$(V; $\pi \rightarrow \pi^\star$) | 3.43 | 3.48 | 3.38 | 3.45 | 3.07 |
| | $^3B_2$(R; $n \rightarrow 4s$) | 5.72 | 5.64 | 5.72 | 5.62 | 5.71 |
| | $^1A_2$[F](V; $n \rightarrow \pi^\star$) | 1.95 | 2.09 | 1.97 | 1.92 | 1.80 |
| Thiophene | $^1A_1$(V; $\pi \rightarrow \pi^\star$) | 5.64 | 5.75 | 5.65 | 5.72 | 5.61 |
| | $^1B_2$(V; $\pi \rightarrow \pi^\star$) | 5.98 | 6.07 | 5.96 | 6.07 | 5.79 |
| | $^1A_2$(R; $\pi \rightarrow 3s$) | 6.14 | 6.07 | 6.14 | 6.15 | 6.03 |
| | $^1B_1$(R; $\pi \rightarrow 3p$) | 6.14 | 6.15 | 6.14 | 6.24 | 6.02 |
| | $^1A_2$(R; $\pi \rightarrow 3p$) | 6.21 | 6.35 | 6.25 | 6.35 | 6.14 |
| | $^1B_1$(R; $\pi \rightarrow 3s$) | 6.49 | 6.48 | 6.50 | 6.51 | 6.43 |
| | $^1B_2$(R; $\pi \rightarrow 3p$) | 7.29 | 7.26 | 7.29 | 7.34 | 7.18 |
| | $^3B_2$(V; $\pi \rightarrow \pi^\star$) | 3.92 | 4.12 | 3.94 | 4.11 | 3.65 |
| | $^3A_1$(V; $\pi \rightarrow \pi^\star$) | 4.76 | 4.91 | 4.77 | 4.86 | 4.56 |
| | $^3B_1$(R; $\pi \rightarrow 3p$) | 5.93 | 6.00 | 5.95 | 6.09 | 5.83 |

Continued on next page

| Compound | State | TBE | CC2 | CC3 | ADC(2) | ADC(3) |
|---|---|---|---|---|---|---|
| | $^3A_2(\mathrm{R}; \pi \to 3s)$ | 6.08 | 6.03 | 6.09 | 6.11 | 5.97 |
| Thiopropynal | $^1A''(\mathrm{V}; n \to \pi^\star)$ | 2.03 | 2.20 | 2.05 | 2.08 | 1.86 |
| | $^3A''(\mathrm{V}; n \to \pi^\star)$ | 1.80 | 1.84 | 1.81 | 1.74 | 1.63 |
| Triazine | $^1A''_1(\mathrm{V}; n \to \pi^\star)$ | 4.72 | 4.64 | 4.73 | 4.58 | 4.83 |
| | $^1A''_2(\mathrm{V}; n \to \pi^\star)$ | 4.75 | 4.75 | 4.74 | 4.69 | 4.99 |
| | $^1E''(\mathrm{V}; n \to \pi^\star)$ | 4.78 | 4.72 | 4.78 | 4.66 | 4.95 |
| | $^1A'_2(\mathrm{V}; \pi \to \pi^\star)$ | 5.75 | 5.89 | 5.78 | 5.83 | 5.78 |
| | $^1A'_1(\mathrm{V}; \pi \to \pi^\star)$ | 7.24 | 7.32 | 7.24 | 7.18 | 6.78 |
| | $^1E'(\mathrm{R}; n \to 3s)$ | 7.32 | 6.87 | 7.35 | 6.89 | 7.68 |
| | $^1E''(\mathrm{V}; n \to \pi^\star)$ | 7.78 | 7.71 | 7.79 | | |
| | $^1E'(\mathrm{V}; \pi \to \pi^\star)$ | 7.94 | 7.63 | 7.92 | 7.65 | 7.88 |
| | $^3A''_2(\mathrm{V}; n \to \pi^\star)$ | 4.33 | 4.32 | 4.33 | 4.29 | 4.35 |
| | $^3E''(\mathrm{V}; n \to \pi^\star)$ | 4.51 | 4.46 | 4.51 | 4.42 | 4.59 |
| | $^3A''_1(\mathrm{V}; n \to \pi^\star)$ | 4.73 | 4.65 | 4.75 | 4.59 | 4.53 |
| | $^3A'_1(\mathrm{V}; \pi \to \pi^\star)$ | 4.85 | 5.12 | 4.88 | 5.10 | 4.97 |
| | $^3E'(\mathrm{V}; \pi \to \pi^\star)$ | 5.59 | 5.88 | 5.61 | 5.82 | 5.32 |
| | $^3A'_2(\mathrm{V}; (\pi \to \pi^\star)$ | 6.62 | 6.76 | 6.63 | 6.63 | 6.27 |
| Water | $^1B_1(\mathrm{R}; n \to 3s)$ | 7.62 | 7.23 | 7.65 | 7.18 | 7.84 |
| | $^1A_2(\mathrm{R}; n \to 3p)$ | 9.41 | 8.89 | 9.43 | 8.84 | 9.63 |
| | $^1A_1(\mathrm{R}; n \to 3s)$ | 9.99 | 9.58 | 10.00 | 9.52 | 10.22 |
| | $^3B_1(\mathrm{R}; n \to 3s)$ | 7.25 | 6.91 | 7.28 | 6.86 | 7.41 |
| | $^3A_2(\mathrm{R}; n \to 3p)$ | 9.24 | 8.77 | 9.26 | 8.72 | 9.43 |
| | $^3A_1(\mathrm{R}; n \to 3s)$ | 9.54 | 9.20 | 9.56 | 9.15 | 9.70 |

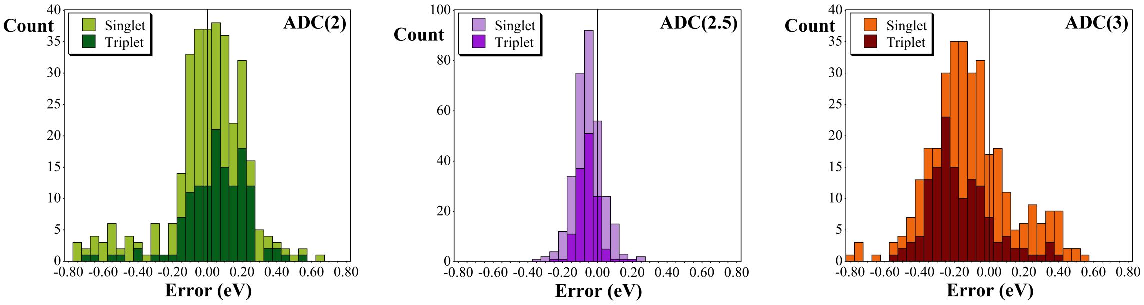


Figure S1: Histograms of the errors (in eV) obtained with ADC(2), ADC(2.5), and ADC(3) taking the TBE/*aug*-cc-pVTZ values of Refs. 1 and 2 as reference (as in Fig. 1 in the main text). "Count" refers to the number of transitions in each group. Note the difference of scaling in the vertical axes.

# 0-0 energies

For the 0-0 energies, we used the (EOM-)CCSD/*def2*-TZVPP geometries available in the Supporting Information of Ref. 3. We reproduce below the experimental values together with the literature references and the ZPVE corrections (mostly determined at the B3LYP/6-31+G(d) level, see Ref. 3 for details). Two "large" (10 non-hydrogen atoms) molecules have been added to the original set: *p*-diisocyano-benzene and tetrafluorobenzene. The geometries are given below in the same format as in Ref. 3.

**Table S2: Experimental 0-0 energies and symmetries for the set of 0-0 energies. The experimental 0-0 energies are reported in both $cm^{-1}$ (the unit used in most experimental works) and eV. The ZPVE are also indicated in eV in the rightmost column.**

| | | Experimental reference | | | |
|---|---|---|---|---|---|
| Molecule | State | $cm^{-1}$ | eV | Ref. | $\Delta^{ZPVE}$ |
| Acetaldehyde | $^1A''$ $(n \to \pi^\star)$ | 29769 | 3.691 | 4 | -0.070 |
| Acetone | $^1A_2$ $(n \to \pi^\star)$ | 30435 | 3.773 | 5 | -0.058 |
| Acetyl cyanide | $^1A''$ $(n \to \pi^\star)$ | 27511 | 3.411 | 6 | -0.053 |
| Acetylene | $^1\Sigma_u^-$ $(\pi \to \pi^\star)$ | 42197.7 | 5.232 | 7 | -0.077 |
| | $^1\Delta_u$ $(\pi \to \pi^\star)$ | 54116 | 6.710 | 8 | -0.136 |
| Acrolein | $^1A''$ $(n \to \pi^\star)$ | 25858.1 | 3.206 | 9 | -0.089 |
| Aniline | $^1A''$ $(\pi \to \pi^\star)$ | 34029 | 4.219 | 10 | -0.191 |
| Benzene | $^1B_{2u}$ $(\pi \to \pi^\star)$ | 38086.7 | 4.722 | 11 | -0.162 |
| Benzonitrile | $^1B_1$ $(\pi \to \pi^\star)$ | 36513 | 4.527 | 12 | -0.145 |
| Benzoquinone | $^1B_{1g}$ $(n \to \pi^\star)$ | 20045 | 2.485 | 13 | -0.080 |
| $CCl_2$ | $^1B_1$ | 17256.9 | 2.140 | 14 | 0.010 |
| CClF | $^1A''$ | 25277.8 | 3.134 | 15 | -0.001 |
| $CF_2$ | $^1B_1$ | 37226 | 4.615 | 16 | -0.008 |
| Cyanoacetylene | $^1\Sigma^-$ $(\pi \to \pi^\star)$ | 38484.9 | 4.772 | 17 | -0.118 |
| | $^1\Delta$ $(\pi \to \pi^\star)$ | 44221 | 5.483 | 18 | -0.119 |
| Cyanoformaldehyde | $^1A''$ $(n \to \pi^\star)$ | 26283.37 | 3.259 | 19 | -0.063 |
| Cyanogen | $^1\Sigma_u^-$ $(\pi \to \pi^\star)$ | 45399.85 | 5.629 | 20 | -0.086 |
| | $^1\Delta_u$ $(\pi \to \pi^\star)$ | | 5.96 | 21 | -0.078 |
| 2-Cyclopenten-1-one | $^1A''$ $(n \to \pi^\star)$ | 27210 | 3.374 | 22 | -0.096 |
| Diacetylene | $^1\Sigma_u^-$ $(\pi \to \pi^\star)$ | 34912.37 | 4.329 | 23 | -0.125 |
| | $^1\Delta_u$ $(\pi \to \pi^\star)$ | 40845 | 5.064 | 24 | -0.192 |
| *p*-Dicyano-benzene | $^1B_{2u}$ $(\pi \to \pi^\star)$ | 35120 | 4.354 | 25 | -0.140 |
| *p*-Diethynylbenzene | $^1B_{2u}$ $(\pi \to \pi^\star)$ | 34255 | 4.247 | 26 | -0.134 |
| *p*-Difluoro-benzene | $^1B_{2u}$ $(\pi \to \pi^\star)$ | 36838 | 4.567 | 27 | -0.160 |
| Difluorodiazirine | $^1B_1$ $(n \to \pi^\star)$ | 28374.21 | 3.518 | 28 | -0.072 |
| 2,6-Difluoro-pyridine | $^1B_2$ $(\pi \to \pi^\star)$ | 37820 | 4.689 | 29 | -0.149 |
| *p*-Diisocyano-benzene | $^1B_{2u}$ $(\pi \to \pi^\star)$ | 35566 | 4.410 | 30 | -0.137 |
| Fluoro-benzene | $^1B_2$ $(\pi \to \pi^\star)$ | 37813 | 4.688 | 31 | -0.161 |

Continued on next page

| Molecule | State | Experimental reference cm$^{-1}$ | eV | Ref. | $\Delta^{\mathrm{ZPVE}}$ |
|---|---|---|---|---|---|
| Formaldehyde | $^1A_2$ $(n \to \pi^\star)$ | 28188.02 | 3.495 | 32 | -0.085 |
| Formic acid | $^1A''$ $(n \to \pi^\star)$ | 37413.39 | 4.639 | 33 | -0.096 |
| Formylchloride | $^1A''$ $(n \to \pi^\star)$ | 32760 | 4.062 | 34 | -0.069 |
| Formylfluoride | $^1A''$ $(n \to \pi^\star)$ | 37491.7 | 4.648 | 35 | -0.063 |
| Glyoxal | $^1A_u$ $(n \to \pi^\star)$ | 21973.43 | 2.724 | 36 | -0.060 |
| $H_2C_3$ | $^1A_2$ $(\pi \to \pi^\star)$ | 13677 | 1.696 | 37 | -0.059 |
| HCN | $^1\Sigma^-$ $(\pi \to \pi^\star)$ | 52256.4 | 6.479 | 7 | -0.120 |
| HCP | $^1\Sigma^-$ $(\pi \to \pi^\star)$ | 34769.9 | 4.311 | 7 | -0.087 |
| HNO | $^1A''$ $(n \to \pi^\star)$ | 13154.4 | 1.631 | 7 | -0.029 |
| HPO | $^1A''$ $(n \to \pi^\star)$ | 19032.78 | 2.360 | 38 | -0.043 |
| HPS | $^1A''$ $(\sigma \to \pi^\star)$ | 12291.4 | 1.524 | 39 | -0.019 |
| HSiF | $^1A''$ | 23260.021 | 2.884 | 40 | -0.037 |
| *cis*-Hydroquinone | $^1A_1$ $(\pi \to \pi^\star)$ | 33534.782 | 4.158 | 41 | -0.156 |
| *trans*-Hydroquinone | $^1B_u$ $(\pi \to \pi^\star)$ | 33500.054 | 4.153 | 41 | -0.159 |
| Isocyanogen | $^1\Sigma^-$ $(\pi \to \pi^\star)$ | 42523 | 5.272 | 42 | -0.077 |
| Nitrosomethane | $^1A''$ $(n \to \pi^\star)$ | 14408 | 1.786 | 43 | -0.026 |
| Nitrosylcyanide | $^1A''$ $(n \to \pi^\star)$ | 11339.9 | 1.406 | 44 | 0.004 |
| Oxalyl fluoride | $^1A_u$ $(n \to \pi^\star)$ | 32445 | 4.023 | 45 | -0.104 |
| Phenylacetylene | $^1B_2$ $(\pi \to \pi^\star)$ | 35877.18 | 4.448 | 46 | -0.158 |
| Phosgene | $^1A_2$ $(n \to \pi^\star)$ | 32730 | 4.058 | 47 | -0.089 |
| Propynal | $^1A''$ $(n \to \pi^\star)$ | 26162.94 | 3.244 | 48 | -0.092 |
| 4H-pyran-4-one | $^1A^2$ $(n \to \pi^\star)$ | 28360 | 3.516 | 49 | -0.122 |
| Pyrazine | $^1B_{3u}$ $(n \to \pi^\star)$ | 30875.78 | 3.828 | 50 | -0.209 |
| Pyrimidine | $^1B_1$ $(n \to p)$ | 31188 | 3.867 | 51 | -0.174 |
| Selenoformaldehyde | $^1A_2$ $(n \to \pi^\star)$ | 13635 | 1.691 | 52 | -0.062 |
| $SiCl_2$ | $^1B_1$ | 30013.5 | 3.721 | 53 | -0.015 |
| Silylidene | $^1A_2$ (Ryd) | 15132.97 | 1.876 | 54 | 0.009 |
| | $^1B_2$ (Ryd) | 29312.88 | 3.634 | 55 | 0.018 |
| Tetrafluorobenzene | $^1B_{2u}$ $(\pi \to \pi^\star)$ | 36555 | 4.532 | 56 | -0.136 |
| Tetrazine | $^1B_{3u}$ $(n \to \pi^\star)$ | 18128.07 | 2.248 | 57 | -0.093 |
| Thioacetaldehyde | $^1A''$ $(n \to \pi^\star)$ | | 2.22 | 58 | -0.064 |
| Thioacetone | $^1A_2$ $(n \to \pi^\star)$ | | 2.33 | 58 | -0.047 |
| Thioacrolein | $^1A''$ $(n \to \pi^\star)$ | 15124.6 | 1.875 | 59 | -0.050 |
| Thiocarbonyllbromide | $^1A_2$ $(n \to \pi^\star)$ | 17992 | 2.231 | 60 | -0.033 |
| Thiocarbonylchlorofluoride | $^1A''$ $(n \to \pi^\star)$ | 21657.4 | 2.685 | 61 | -0.032 |
| | $^2A'$ $(\pi \to \pi^\star)$ | 35277 | 4.374 | 62 | -0.066 |
| Thiocarbonylfluoride | $^1A_2$ $(n \to \pi^\star)$ | 23477.1 | 2.911 | 63 | -0.034 |
| Thioformaldehyde | $^1A_2$ $(n \to \pi^\star)$ | 16395.6 | 2.033 | 32 | -0.066 |
| Thioformylchloride | $^1A''$ $(n \to \pi^\star)$ | 18792 | 2.330 | 64 | -0.054 |
| Thiophosgene | $^1A_2$ $(n \to \pi^\star)$ | 18712.2 | 2.320 | 65 | -0.030 |
| | $^2A_1$ $(\pi \to \pi^\star)$ | 34277.32 | 4.250 | 65 | -0.069 |
| Thiopropynal | $^1A''$ $(n \to \pi^\star)$ | 14656.4 | 1.817 | 66 | -0.048 |
| Trifluoronitrosomethane | $^1A''$ $(n \to \pi^\star)$ | 13929.7 | 1.727 | 67 | -0.017 |
| Acetaldehyde | $^3A''$ $(n \to \pi^\star)$ | 27240 | 3.377 | 68 | -0.074 |
| Acrolein | $^3A''$ $(n \to \pi^\star)$ | 24247.3 | 3.006 | 69 | -0.109 |
| Benzaldehyde | $^3A''$ $(n \to \pi^\star)$ | 25183 | 3.122 | 70 | -0.111 |
| Benzoquinone | $^3B_{1g}$ $(n \to \pi^\star)$ | 18370 | 2.278 | 71 | -0.075 |

Continued on next page

| Molecule | State | Experimental reference cm$^{-1}$ | eV | Ref. | $\Delta^{\text{ZPVE}}$ |
|---|---|---|---|---|---|
| CHCl | $^3A''$ | 2163.28 | 0.268 | 72 | 0.007 |
| Cyanogen | $^3\Sigma_u^+$ $(\pi \rightarrow \pi^\star)$ | 33289.9 | 4.127 | 73 | -0.110 |
| 4-Cyclopentene-1,3-dione | $^3B_1$ $(n \rightarrow \pi^\star)$ | 20540 | 2.547 | 74 | -0.074 |
| 2-Cyclopenten-1-one | $^3A''$ $(n \rightarrow \pi^\star)$ | 25956.29 | 3.218 | 75 | -0.111 |
| Formaldehyde | $^3A_2$ $(n \rightarrow \pi^\star)$ | 25194.34 | 3.124 | 32 | -0.092 |
| Glyoxal | $^3A_u$ $(n \rightarrow \pi^\star)$ | 19199 | 2.380 | 76 | -0.056 |
| $H_2C_3$ | $^3B_1$ $(\pi \rightarrow \pi^\star)$ | 10354 | 1.284 | 37 | -0.066 |
| Oxalyl Chloride | $^3A_u$ $(n \rightarrow \pi^\star)$ | 410.02[a] | 3.024 | 77 | -0.085 |
| Ozone | $^3A_2$ | 9553.021 | 1.184 | 78 | -0.061 |
| Propynal | $^3A''$ $(n \rightarrow \pi^\star)$ | 24127.1 | 2.991 | 79 | -0.106 |
| 4H-pyran-4-one | $^3A^2$ $(n \rightarrow \pi^\star)$ | 27291.5 | 3.384 | 80 | -0.134 |
| 4H-pyran-4-thione | $^3A^2$ $(n \rightarrow \pi^\star)$ | 16846.4 | 2.089 | 81 | -0.097 |
| Pyrazine | $^3B_{3u}$ $(n \rightarrow \pi^\star)$ | 26820.3 | 3.325 | 82 | -0.177 |
| Pyrimidine | $^3B_1$ $(n \rightarrow \pi^\star)$ | 28534.0 | 3.538 | 83 | -0.176 |
| Selenoformaldehyde | $^3A_2$ $(n \rightarrow \pi^\star)$ | 12171.0 | 1.509 | 84 | -0.071 |
| $SiF_2$ | $^3B_1$ | 26319.5 | 3.263 | 85 | -0.002 |
| $SO_2$ | $^3B_1$ | 25765.737 | 3.195 | 86 | -0.055 |
| Tetrazine | $^3B_{3u}$ $(n \rightarrow \pi^\star)$ | 13608.0 | 1.687 | 87 | -0.061 |
| Thioacetaldehyde | $^3A''$ $(n \rightarrow \pi^\star)$ | 16293.8 | 2.020 | 88 | -0.060 |
| Thioacetone | $^3A_2$ $(n \rightarrow \pi^\star)$ | 17327.8 | 2.148 | 89 | -0.045 |
| Thioacrolein | $^3A''$ $(n \rightarrow \pi^\star)$ | 14036.2 | 1.740 | 59 | -0.070 |
| Thioformaldehyde | $^3A_2$ $(n \rightarrow \pi^\star)$ | 14507.39 | 1.799 | 32 | -0.080 |
| Thioformylchloride | $^3A''$ $(n \rightarrow \pi^\star)$ | 17233.9 | 2.137 | 64 | -0.050 |
| Thiophosgene | $^3A_2$ $(n \rightarrow \pi^\star)$ | 17493.788 | 2.169 | 90 | -0.035 |
| Thiopropynal | $^1A''$ $(n \rightarrow \pi^\star)$ | 13257.4 | 1.644 | 66 | -0.064 |
| Triazine | $^3E$" $(n \rightarrow \pi^\star)$ | 335[a,b] | 3.701 | 91 | -0.148 |

[a] in nm; [b] "best estimate"

Cartesian coordinates (in Å) obtained at the (EOM-)CCSD/*def2*-TZVPP level of theory for the two additional compounds. The notations of the excited states refer to the ground-state point group symmetry.

### ***p*-Diisocyano-benzene**

Ground state

```
C        0.000000    1.210459    0.692565
C        0.000000    1.210459   -0.692565
C        0.000000    0.000000    1.377022
C        0.000000    0.000000   -1.377022
C        0.000000   -1.210459    0.692565
C        0.000000   -1.210459   -0.692565
C        0.000000    0.000000    3.932314
```

| | | | |
|---|---|---|---|
| C | 0.000000 | 0.000000 | -3.932314 |
| N | 0.000000 | 0.000000 | 2.763434 |
| N | 0.000000 | 0.000000 | -2.763434 |
| H | 0.000000 | 2.135125 | 1.244480 |
| H | 0.000000 | 2.135125 | -1.244480 |
| H | 0.000000 | -2.135125 | 1.244480 |
| H | 0.000000 | -2.135125 | -1.244480 |

Excited state [$^1B_{2u}$ ($\pi \rightarrow \pi^\star$)]

| | | | |
|---|---|---|---|
| C | 0.000000 | 1.238754 | 0.709424 |
| C | 0.000000 | 1.238754 | -0.709424 |
| C | 0.000000 | -0.000000 | 1.404087 |
| C | 0.000000 | -0.000000 | -1.404087 |
| C | 0.000000 | -1.238754 | 0.709424 |
| C | 0.000000 | -1.238754 | -0.709424 |
| C | 0.000000 | -0.000000 | 3.944346 |
| C | 0.000000 | -0.000000 | -3.944346 |
| N | 0.000000 | -0.000000 | 2.771103 |
| N | 0.000000 | -0.000000 | -2.771103 |
| H | 0.000000 | 2.159635 | 1.265112 |
| H | 0.000000 | 2.159635 | -1.265112 |
| H | 0.000000 | -2.159635 | 1.265112 |
| H | 0.000000 | -2.159635 | -1.265112 |

**Tetrafluorobenzene**

Ground state

| | | | |
|---|---|---|---|
| C | 0.000000 | 1.190995 | 0.692100 |
| C | 0.000000 | 1.190995 | -0.692100 |
| C | 0.000000 | 0.000000 | -1.393333 |
| C | 0.000000 | -1.190995 | -0.692100 |
| C | 0.000000 | -1.190995 | 0.692100 |
| C | 0.000000 | 0.000000 | 1.393333 |
| F | 0.000000 | 2.348323 | -1.348963 |
| F | 0.000000 | 2.348323 | 1.348963 |
| F | 0.000000 | -2.348323 | 1.348963 |
| F | 0.000000 | -2.348323 | -1.348963 |
| H | 0.000000 | 0.000000 | -2.469482 |
| H | 0.000000 | 0.000000 | 2.469482 |

Excited state [$^1B_{2u}$ ($\pi \rightarrow \pi^\star$)]

| | | | |
|---|---|---|---|
| C | 1.178195 | 0.707583 | 0.063424 |
| C | 1.178195 | -0.707583 | 0.063424 |
| C | 0.000000 | -1.473594 | 0.163267 |

| | | | |
|---|---|---|---|
| C | -1.178195 | -0.707583 | 0.063424 |
| C | -1.178195 | 0.707583 | 0.063424 |
| C | 0.000000 | 1.473594 | 0.163267 |
| F | 2.339183 | -1.319369 | -0.118329 |
| F | 2.339183 | 1.319369 | -0.118329 |
| F | -2.339183 | 1.319369 | -0.118329 |
| F | -2.339183 | -1.319369 | -0.118329 |
| H | 0.000000 | -2.523792 | 0.389226 |
| H | 0.000000 | 2.523792 | 0.389226 |

**Table S3: 0-0 energies computed with ADC(2), ADC(3), CC2, and CC3. All values are in eV, and they have been obtained on the basis of the corresponding *aug*-cc-pVTZ frozen-core adiabatic energies determined on the (EOM-)CCSD/*def2*-TZVPP geometries. The ZPVE corrections are listed above.**

| Molecule | State | ADC(2) | ADC(3) | CC2 | CC3 |
|---|---|---|---|---|---|
| Acetaldehyde | $^1A''$ $(n \to \pi^\star)$ | 3.455 | 3.830 | 3.671 | 3.663 |
| Acetone | $^1A_2$ $(n \to \pi^\star)$ | 3.430 | 4.007 | 3.671 | 3.733 |
| Acetyl cyanide | $^1A''$ $(n \to \pi^\star)$ | 3.136 | 3.607 | 3.348 | 3.381 |
| Acetylene | $^1\Sigma_u^-$ $(\pi \to \pi^\star)$ | 5.323 | 4.753 | 5.322 | 5.163 |
| | $^1\Delta_u$ $(\pi \to \pi^\star)$ | 6.797 | 6.247 | 6.808 | 6.627 |
| Acrolein | $^1A''$ $(n \to \pi^\star)$ | 3.040 | 3.445 | 3.254 | 3.229 |
| Aniline | $^1A''$ $(\pi \to \pi^\star)$ | 4.264 | 4.165 | 4.261 | 4.169 |
| Benzene | $^1B_{2u}$ $(\pi \to \pi^\star)$ | 4.930 | 4.684 | 4.904 | 4.709 |
| Benzonitrile | $^1B_1$ $(\pi \to \pi^\star)$ | 4.735 | 4.494 | 4.711 | 4.526 |
| Benzoquinone | $^1B_{1g}$ $(n \to \pi^\star)$ | 2.310 | 2.788 | 2.443 | 2.502 |
| $CCl_2$ | $^1B_1$ | 2.066 | 1.986 | 2.180 | 2.232 |
| CClF | $^1A''$ | 3.048 | 2.978 | 3.170 | 3.198 |
| $CF_2$ | $^1B_1$ | 4.504 | 4.474 | 4.632 | 4.642 |
| Cyanoacetylene | $^1\Sigma^-$ $(\pi \to \pi^\star)$ | 4.815 | 4.323 | 4.780 | 4.693 |
| | $^1\Delta$ $(\pi \to \pi^\star)$ | 5.483 | 5.060 | 5.480 | 5.413 |
| Cyanoformaldehyde | $^1A''$ $(n \to \pi^\star)$ | 3.133 | 3.371 | 3.309 | 3.270 |
| Cyanogen | $^1\Sigma_u^-$ $(\pi \to \pi^\star)$ | 5.721 | 5.212 | 5.696 | 5.595 |
| | $^1\Delta_u$ $(\pi \to \pi^\star)$ | 6.051 | 5.529 | 6.045 | 5.907 |
| 2-Cyclopenten-1-one | $^1A''$ $(n \to \pi^\star)$ | 3.065 | 3.734 | 3.275 | 3.355 |
| Diacetylene | $^1\Sigma_u^-$ $(\pi \to \pi^\star)$ | 4.268 | 3.927 | 4.237 | 4.243 |
| | $^1\Delta_u$ $(\pi \to \pi^\star)$ | 4.966 | 4.613 | 4.958 | 4.935 |
| *p*-Dicyano-benzene | $^1B_{2u}$ $(\pi \to \pi^\star)$ | 4.546 | 4.308 | 4.522 | 4.351 |
| *p*-Diethynylbenzene | $^1B_{2u}$ $(\pi \to \pi^\star)$ | 4.455 | 4.220 | 4.434 | 4.265 |
| *p*-Difluoro-benzene | $^1B_{2u}$ $(\pi \to \pi^\star)$ | 4.631 | 4.519 | 4.741 | 4.525 |
| Difluorodiazirine | $^1B_1$ $(n \to \pi^\star)$ | 3.488 | 3.304 | 3.477 | 3.501 |
| 2,6-Difluoro-pyridine | $^1B_2$ $(\pi \to \pi^\star)$ | 4.744 | 4.647 | 4.758 | 4.644 |
| *p*-Diisocyano-benzene | $^1B_{2u}$ $(\pi \to \pi^\star)$ | 4.606 | 4.372 | 4.590 | 4.407 |
| Fluoro-benzene | $^1B_2$ $(\pi \to \pi^\star)$ | 4.841 | 4.648 | 4.831 | 4.664 |
| Formaldehyde | $^1A_2$ $(n \to \pi^\star)$ | 3.365 | 3.548 | 3.541 | 3.482 |
| Formic acid | $^1A''$ $(n \to \pi^\star)$ | 4.308 | 4.886 | 4.563 | 4.588 |
| Formylchloride | $^1A''$ $(n \to \pi^\star)$ | 3.839 | 4.219 | 4.075 | 4.047 |
| Formylfluoride | $^1A''$ $(n \to \pi^\star)$ | 4.410 | 4.820 | 4.661 | 4.611 |
| Glyoxal | $^1A_u$ $(n \to \pi^\star)$ | 2.662 | 2.733 | 2.727 | 2.726 |
| $H_2C_3$ | $^1A_2$ $(\pi \to \pi^\star)$ | 1.952 | 1.418 | 1.930 | 1.713 |
| HCN | $^1\Sigma^-$ $(\pi \to \pi^\star)$ | 6.760 | 5.963 | 6.681 | 6.409 |
| HCP | $^1\Sigma^-$ $(\pi \to \pi^\star)$ | 4.458 | 3.794 | 4.432 | 4.250 |
| HNO | $^1A''$ $(n \to \pi^\star)$ | 1.555 | 1.403 | 1.600 | 1.637 |
| HPO | $^1A''$ $(n \to \pi^\star)$ | 2.087 | 2.291 | 2.242 | 2.277 |
| HPS | $^1A''$ $(\sigma \to \pi^\star)$ | 1.460 | 1.250 | 1.522 | 1.426 |
| HSiF | $^1A''$ | 2.923 | 2.684 | 2.955 | 2.886 |
| *cis*-Hydroquinone | $^1A_1$ $(\pi \to \pi^\star)$ | 4.119 | 4.103 | 4.125 | 4.092 |
| *trans*-Hydroquinone | $^1B_u$ $(\pi \to \pi^\star)$ | 4.111 | 4.097 | 4.127 | 4.085 |

Continued on next page

| Molecule | State | ADC(2) | ADC(3) | CC2 | CC3 |
|---|---|---|---|---|---|
| Isocyanogen | $^1\Sigma^-$ ($\pi \rightarrow \pi^\star$) | 5.209 | 5.168 | 5.405 | 5.108 |
| Nitrosomethane | $^1A''$ ($n \rightarrow \pi^\star$) | 1.666 | 1.569 | 1.749 | 1.781 |
| Nitrosylcyanide | $^1A''$ ($n \rightarrow \pi^\star$) | 1.441 | 1.165 | 1.417 | 1.446 |
| Oxalyl fluoride | $^1A_u$ ($n \rightarrow \pi^\star$) | 3.758 | 4.209 | 3.928 | 3.988 |
| Phenylacetylene | $^1B_2$ ($\pi \rightarrow \pi^\star$) | 4.652 | 4.409 | 4.628 | 4.445 |
| Phosgene | $^1A_2$ ($n \rightarrow \pi^\star$) | 3.727 | 4.394 | 3.956 | 4.039 |
| Propynal | $^1A''$ ($n \rightarrow \pi^\star$) | 3.039 | 3.430 | 3.251 | 3.241 |
| 4H-pyran-4-one | $^1A^2$ ($n \rightarrow \pi^\star$) | 3.168 | 3.971 | 3.422 | 3.487 |
| Pyrazine | $^1B_{3u}$ ($n \rightarrow \pi^\star$) | 3.827 | 3.797 | 3.795 | 3.799 |
| Pyrimidine | $^1B_1$ ($n \rightarrow p$) | 3.717 | 3.909 | 3.770 | 3.818 |
| Selenoformaldehyde | $^1A_2$ ($n \rightarrow \pi^\star$) | 1.659 | 1.625 | 1.812 | 1.708 |
| $SiCl_2$ | $^1B_1$ | 3.749 | 3.541 | 3.794 | 3.697 |
| Silylidene | $^1A_2$ (Ryd) | 2.127 | 1.557 | 2.089 | 1.850 |
| | $^1B_2$ (Ryd) | 3.692 | 3.224 | 3.633 | 3.579 |
| Tetrafluorobenzene | $^1B_{2u}$ ($\pi \rightarrow \pi^\star$) | 4.532 | 4.501 | 4.553 | 4.487 |
| Tetrazine | $^1B_{3u}$ ($n \rightarrow \pi^\star$) | 2.207 | 2.185 | 2.177 | 2.246 |
| Thioacetaldehyde | $^1A''$ ($n \rightarrow \pi^\star$) | 2.145 | 2.169 | 2.300 | 2.204 |
| Thioacetone | $^1A_2$ ($n \rightarrow \pi^\star$) | 2.171 | 2.361 | 2.358 | 2.298 |
| Thioacrolein | $^1A''$ ($n \rightarrow \pi^\star$) | 1.913 | 1.828 | 2.062 | 1.923 |
| Thiocarbonyllbromide | $^1A_2$ ($n \rightarrow \pi^\star$) | 2.114 | 2.237 | 2.284 | 2.233 |
| Thiocarbonylchlorofluoride | $^1A''$ ($n \rightarrow \pi^\star$) | 2.582 | 2.640 | 2.756 | 2.618 |
| | $^2A'$ ($\pi \rightarrow \pi^\star$) | 4.112 | 4.007 | 4.542 | 4.324 |
| Thiocarbonylfluoride | $^1A_2$ ($n \rightarrow \pi^\star$) | 2.889 | 2.825 | 3.029 | 2.815 |
| Thioformaldehyde | $^1A_2$ ($n \rightarrow \pi^\star$) | 2.042 | 1.911 | 2.154 | 2.038 |
| Thioformylchloride | $^1A''$ ($n \rightarrow \pi^\star$) | 2.282 | 2.277 | 2.448 | 2.337 |
| Thiophosgene | $^1A_2$ ($n \rightarrow \pi^\star$) | 2.240 | 2.368 | 2.425 | 2.349 |
| | $^2A_1$ ($\pi \rightarrow \pi^\star$) | 3.948 | 3.878 | 4.411 | 4.229 |
| Thiopropynal | $^1A''$ ($n \rightarrow \pi^\star$) | 1.845 | 1.715 | 1.971 | 1.849 |
| Trifluoronitrosomethane | $^1A''$ ($n \rightarrow \pi^\star$) | 1.666 | 1.470 | 1.717 | 1.739 |
| Acetaldehyde | $^3A''$ ($n \rightarrow \pi^\star$) | 3.037 | 3.429 | 3.214 | 3.308 |
| Acrolein | $^3A''$ ($n \rightarrow \pi^\star$) | 2.664 | 3.172 | 2.849 | 2.946 |
| Benzaldehyde | $^3A''$ ($n \rightarrow \pi^\star$) | 2.711 | 3.333 | 2.900 | 3.050 |
| Benzoquinone | $^3B_{1g}$ ($n \rightarrow \pi^\star$) | 2.161 | 2.522 | 2.229 | 2.351 |
| CHCl | $^3A''$ | 0.091 | 0.010 | 0.190 | 0.270 |
| Cyanogen | $^3\Sigma_u^+$ ($\pi \rightarrow \pi^\star$) | 4.329 | 3.790 | 4.263 | 4.006 |
| 4-Cyclopentene-1,3-dione | $^3B_1$ ($n \rightarrow \pi^\star$) | 2.219 | 2.765 | 2.297 | 2.499 |
| 2-Cyclopenten-1-one | $^3A''$ ($n \rightarrow \pi^\star$) | 2.767 | 3.549 | 2.960 | 3.137 |
| Formaldehyde | $^3A_2$ ($n \rightarrow \pi^\star$) | 2.878 | 3.092 | 3.012 | 3.067 |
| Glyoxal | $^3A_u$ ($n \rightarrow \pi^\star$) | 2.247 | 2.320 | 2.308 | 2.360 |
| $H_2C_3$ | $^3B_1$ ($\pi \rightarrow \pi^\star$) | 1.395 | 1.115 | 1.378 | 1.308 |
| Oxalyl Chloride | $^3A_u$ ($n \rightarrow \pi^\star$) | 2.663 | 3.238 | 2.808 | 3.004 |
| Ozone | $^3A_2$ | 1.377 | 0.459 | 1.051 | 1.164 |
| Propynal | $^3A''$ ($n \rightarrow \pi^\star$) | 2.628 | 3.104 | 2.804 | 2.922 |
| 4H-pyran-4-one | $^3A^2$ ($n \rightarrow \pi^\star$) | 2.892 | 3.770 | 3.122 | 3.293 |
| 4H-pyran-4-thione | $^3A^2$ ($n \rightarrow \pi^\star$) | 1.934 | 2.117 | 2.095 | 2.044 |
| Pyrazine | $^3B_{3u}$ ($n \rightarrow \pi^\star$) | 3.333 | 3.242 | 3.312 | 3.301 |
| Pyrimidine | $^3B_1$ ($n \rightarrow \pi^\star$) | 3.389 | 3.527 | 3.432 | 3.486 |
| Selenoformaldehyde | $^3A_2$ ($n \rightarrow \pi^\star$) | 1.340 | 1.403 | 1.461 | 1.475 |

Continued on next page

| Molecule | State | ADC(2) | ADC(3) | CC2 | CC3 |
|---|---|---|---|---|---|
| $SiF_2$ | $^3B_1$ | 2.932 | 3.019 | 2.992 | 3.176 |
| $SO_2$ | $^3B_1$ | 2.774 | 2.829 | 2.804 | 2.925 |
| Tetrazine | $^3B_{3u}$ $(n \rightarrow \pi^\star)$ | 1.666 | 1.543 | 1.642 | 1.673 |
| Thioacetaldehyde | $^3A^{''}$ $(n \rightarrow \pi^\star)$ | 1.855 | 1.941 | 1.977 | 1.986 |
| Thioacetone | $^3A_2$ $(n \rightarrow \pi^\star)$ | 1.923 | 2.149 | 2.075 | 2.108 |
| Thioacrolein | $^3A^{''}$ $(n \rightarrow \pi^\star)$ | 1.624 | 1.628 | 1.742 | 1.712 |
| Thioformaldehyde | $^3A_2$ $(n \rightarrow \pi^\star)$ | 1.675 | 1.646 | 1.761 | 1.763 |
| Thioformylchloride | $^3A^{''}$ $(n \rightarrow \pi^\star)$ | 1.980 | 2.050 | 2.117 | 2.115 |
| Thiophosgene | $^3A_2$ $(n \rightarrow \pi^\star)$ | 1.960 | 2.158 | 2.117 | 2.141 |
| Thiopropynal | $^1A^{''}$ $(n \rightarrow \pi^\star)$ | 1.515 | 1.501 | 1.613 | 1.613 |
| Triazine | $^3E$" $(n \rightarrow \pi^\star)$ | 3.451 | 3.730 | 3.530 | 3.643 |

# References


(1) Loos, P.-F.; Scemama, A.; Blondel, A.; Garniron, Y.; Caffarel, M.; Jacquemin, D. A Mountaineering Strategy to Excited States: Highly-Accurate Reference Energies and Benchmarks. *J. Chem. Theory Comput.* **2018**, *14*, 4360–4379.

(2) Loos, P.-F.; Lipparini, F.; Boggio-Pasqua, M.; Scemama, A.; Jacquemin, D. A Mountaineering Strategy to Excited States: Highly-Accurate Energies and Benchmarks for Medium Size Molecules. *J. Chem. Theory Comput.* **2020**, *xxxx*, xxx–xxxxx.

(3) Loos, P.-F.; Jacquemin, D. Chemically Accurate 0-0 Energies with not-so-Accurate Excited State Geometries. *J. Chem. Theory Comput.* **2019**, *15*, 2481–2491.

(4) Liu, H.; Lim, E. C.; Judge, R. H.; Moule, D. C. The Hybrid Rotational Components in the $0_0^0$ Origin Band of the $\tilde{A}A'(S_1) \leftarrow \tilde{X}A'(S_0)$ Transition in Acetaldehyde. *J. Chem. Phys.* **1995**, *102*, 4315–4320.

(5) Baba, M.; Hanazaki, I. The $S_1,^1A_2(n,\pi^\star)$ State of Acetone in a Supersonic Nozzle Beam. Methyl Internal Rotation. *Chem. Phys. Lett.* **1983**, *103*, 93–97.

(6) Yoon, M.-C.; Choi, Y. S.; Kim, S. K. Fluorescence Excitation Spectroscopic Study of the Jet-Cooled Acetyl Cyanide. *J. Chem. Phys.* **1999**, *110*, 7185–7191.

(7) Herzberg, G. *Molecular Spectra and Molecular Structure. III. Electronic Spectra and Electronic Structure of Polyatomic Molecules*; D. Van Nostrand Company: London, UK, 1966.

(8) Foo, P.; Innes, K. Spectrum of Acetylene: 1650–1950 Å. *Chem. Phys. Lett.* **1973**, *22*, 439–442.

(9) Hollas, J. The Electronic Absorption Spectrum of Acrolein Vapour. *Spectrochim. Acta* **1963**, *19*, 1425–1441.

(10) Sinclair, W. E.; Pratt, D. W. Structure and vibrational dynamics of aniline and aniline–Ar from high resolution electronic spectroscopy in the gas phase. *J. Chem. Phys.* **1996**, *105*, 7942–7956.

(11) Christiansen, O.; Stanton, J. F.; Gauss, J. A Coupled Cluster Study of the $1^1A_{1g}$ and $1^1B_{2u}$ States of Benzene. *J. Chem. Phys.* **1998**, *108*, 3987–4001.

(12) Borst, D. R.; Pratt, D. W.; Schäfer, M. Molecular recognition in the gas phase. Dipole-bound complexes of benzonitrile with water, ammonia, methanol, acetonitrile, and benzonitrile itself. *Phys. Chem. Chem. Phys.* **2007**, *9*, 4563–4571.

(13) Horst, G. T.; Kommandeur, J. The Singlet $n\pi^\star$ States of para-Benzoquinone. *Chem. Phys.* **1979**, *44*, 287–293.

(14) Richmond, C.; Tao, C.; Mukarakate, C.; Fan, H.; Nauta, K.; Schmidt, T. W.; Kable, S. H.; Reid, S. A. Unraveling the $\tilde{A}^1B_1 \leftarrow \tilde{X}^1A_1$ Spectrum of $CCl_2$: The Renner–Teller Effect, Barrier to Linearity, and Vibrational Analysis Using an Effective Polyad Hamiltonian. *J. Phys. Chem. A* **2008**, *112*, 11355–11362, PMID: 18925733.

(15) Karolczak, J.; Joo, D. L.; Clouthier, D. J. The electronic spectrum of chlorofluorocarbene. *J. Chem. Phys.* **1993**, *99*, 1447–1456.

(16) Mathews, C. W. The Absorption Spectrum of $CF_2$. *Can. J. Phys.* **1967**, *45*, 2355–2374.

(17) Job, V.; King, G. The Electronic Spectrum of Cyanoacetylene: Part I. Analysis of the 2600-Å System. *J. Mol. Spectrosc.* **1966**, *19*, 155–177.

(18) Job, V.; King, G. The Electronic Spectrum of Cyanoacetylene: Part II. Analysis of the 2300-Å System. *J. Mol. Spectrosc.* **1966**, *19*, 178–184.

(19) Karolczak, J.; Clouthier, D. J.; Judge, R.; Moule, D. High-Resolution Absorption and Pyrolysis Jet Spectroscopy of the $0^0_0$ Band of the $\tilde{A}^1A" \leftarrow \tilde{X}^1A"(n \rightarrow \pi^\star)$ Electronic Transition of Formyl Cyanide, HCOCN. *J. Mol. Spectrosc.* **1991**, *147*, 61–70.

(20) Fish, G.; Cartwright, G.; Walsh, A.; Warsop, P. Rotational Structure in the $^1\Sigma_u^- \leftarrow ^1\Sigma_g^+$ Transition of Cyanogen at 2200 Å. *J. Mol. Spectrosc.* **1972**, *41*, 20–32.

(21) Halpern, J. B.; Huang, Y. Radiative Lifetimes, Fluorescence Quantum Yields and Photodissociation of the $C_2N_2$ ($A^1\Sigma_u^-$) and ($B^1\Delta_u$) States: Evidence for Sterically Hindered, Triplet Mediated Crossings to the ($X^1\Sigma_g^+$) Ground State. *Chem. Phys.* **1997**, *222*, 71–86.

(22) Cheatham, C. M.; Laane, J. The Jet-cooled Fluorescence Excitation Spectrum and Ring-Bending Potential-Energy Function and Conformation of 2-Cyclopenten-1-one in the $S_1(n, \pi^\star)$ Electronic Excited State. *J. Chem. Phys.* **1991**, *94*, 7734–7743.

(23) Hardwick, J. L.; Ramsay, D. A. The Near Ultraviolet Band System of Diacetylene. *Chem. Phys. Lett.* **1977**, *48*, 399–401.

(24) Bandy, R. E.; Lakshminarayan, C.; Zwier, T. S. Spectroscopy and Photophysics of the $^1\Delta \leftarrow ^1\Sigma_g^+$ Transition of Jet-Cooled $C_4H_2$, $C_4HD$, and $C_4D_2$. *J. Phys. Chem.* **1992**, *96*, 5337–5343.

(25) Fujita, K.; Fujiwara, T.; Matsunaga, K.; Ono, F.; Nakajima, A.; Watanabe, H.; Koguchi, T.; Suzuka, I.; Matsuzawa, H. a. Electronic spectra of p-dicyanobenzene (p-DCNB), p-DCNB-H2O complex, and p-DCNB dimer in a supersonic jet. *J. Phys. Chem.* **1992**, *96*, 10693–10697.

(26) Stearns, J. A.; Zwier, T. S. Infrared and Ultraviolet Spectroscopy of Jet-Cooled ortho-, meta-, and para-Diethynylbenzene. *J. Phys. Chem. A* **2003**, *107*, 10717–10724.

(27) Knight, A. E. W.; Kable, S. H. The $S_1 - -S_0(^1B_{2u} - -^1Ag)$ transition of p-difluorobenzene cooled in a supersonic free jet expansion. Excitation and dispersed fluorescence spectra, vibrational assignments, Fermi resonances, and forbidden transitions. *J. Chem. Phys.* **1988**, *89*, 7139–7160.

(28) Sieber, H.; Riedle, E.; Neusser, H. Doppler-Free Two-Photon Spectrum of the $0_0^0$ Band of the $\tilde{A}^1B_1 \leftarrow \tilde{X}^1A_1$ Transition in Difluorodiazirine, $F_2CN_2$. *Chem. Phys. Lett.* **1990**, *169*, 191–197.

(29) Nibu, Y.; Okabe, C.; Shimada, H. Observation of Electronic Spectra of Three Isomers of 2,6-Difluoropyridine–Water Clusters. *J. Phys. Chem. A* **2003**, *107*, 1945–1954.

(30) Mehta-Hurt, D. N.; Korn, J. A.; Gutberlet, A. K.; Zwier, T. S. Vibronic Spectroscopy of a Nitrile/Isonitrile Isoelectronic Pair: para-Diisocyanobenzene and para-Isocyanobenzonitrile. *J. Phys. Chem. A* **2015**, *119*, 2863–2877, PMID: 25699407.

(31) Butler, P.; Moss, D. B.; Yin, H.; Schmidt, T. W.; Kable, S. H. Spectroscopy of the $\tilde{A}(^1B_2) - -\tilde{X}(^1A_1)$ transition of jet-cooled fluorobenzene: Laser-induced fluorescence, dispersed fluorescence, and pathological Fermi resonances. *J. Chem. Phys.* **2007**, *127*, 094303.

(32) Clouthier, D. J.; Ramsay, D. A. The Spectroscopy of Formaldehyde and Thioformaldehyde. *Annu. Rev. Phys. Chem.* **1983**, *34*, 31–58.

(33) Beaty-Travis, L. M.; Moule, D. C.; Liu, H.; Lim, E. C.; Judge, R. Analysis of the High-Resolution Rotational Structure of the Origin and First Torsional Members of the 267-nm Band System of Formic Acid. *J. Mol. Spectrosc.* **2001**, *205*, 232–238.

(34) Ding, H.; J. Orr-Ewing, A.; N. Dixon, R. Rotational Structure in the $\tilde{A}^1A" - \tilde{X}^1A'$ Spectrum of Formyl Chloride. *Phys. Chem. Chem. Phys.* **1999**, *1*, 4181–4185.

(35) Crane, J. C.; Nam, H.; Beal, H. P.; Clauberg, H.; Choi, Y. S.; Moore, C.; Stanton, J. F. Vibrational Assignment of the $S_1$ Fluorescence Excitation Spectrum of Formyl Fluoride. *J. Mol. Spectrosc.* **1997**, *181*, 56–66.

(36) Padlus, J.; Ramsay, D. A. The 4550 Å Band System of Glyoxal I. Rotational Analyses of the (0-0) Bands for $C_2H_2O_2$, $C_2HDO_2$, and $C_2D_2O_2$. *Can. J. Phys.* **1967**, *45*, 1389–1412.

(37) Stanton, J. F.; Garand, E.; Kim, J.; Yacovitch, T. I.; Hock, C.; Case, A. S.; Miller, E. M.; Lu, Y.-J.; Vogelhuber, K. M.; Wren, S. W. et al. Ground and Low-Lying Excited States of Propadienylidene ($H_2C{=}C{=}C$:) Obtained by Negative Ion Photoelectron Spectroscopy. *J. Chem. Phys.* **2012**, *136*, 134312.

(38) Tackett, B. S.; Clouthier, D. J. HPO does not follow Walsh's rules! Improved molecular structures from the spectroscopy of jet-cooled HPO and DPO. *J. Chem. Phys.* **2002**, *117*, 10604–10612.

(39) Grimminger, R.; Clouthier, D. J.; Tarroni, R.; Wang, Z.; Sears, T. J. An Experimental and Theoretical Study of the Electronic Spectrum of HPS, a Second row HNO Analog. *J. Chem. Phys.* **2013**, *139*, 174306.

(40) Harper, W. W.; Karolczak, J.; Clouthier, D. J.; Ross, S. C. Chemical reaction jet spectroscopy, molecular structure, and the bending potential of the $\tilde{A}^1A$" state of monofluorosilylene (HSiF). *J. Chem. Phys.* **1995**, *103*, 883–891.

(41) Humphrey, S. J.; Pratt, D. W. High Resolution $S_1 \leftarrow S_0$ Fluorescence Excitation Spectra of Hydroquinone. Distinguishing the *cis* and *trans* Rotamers by their Nuclear Spin Statistical Weights. *J. Chem. Phys.* **1993**, *99*, 5078–5086.

(42) Lynch, W. B.; Bechtel, H. A.; Steeves, A. H.; Curley, J. J.; Field, R. W. Observation of the $\tilde{A}^1A$" State of Isocyanogen. *J. Chem. Phys.* **2007**, *126*, 244307.

(43) Ernsting, N. P.; Pfab, J.; Romelt, J. Geometry Changes Accompanying Electronic Excitation of Nitrosomethane in the 650 nm Region. *J. Chem. Soc., Faraday Trans. 2* **1978**, *74*, 2286–2294.

(44) Dixon, R. N.; Johnson, P. A Rotational Analysis of the $\tilde{A}^1A" - \tilde{X}^1A'$ Electronic Origin Band of NCNO near 882 nm. *J. Mol. Spectrosc.* **1985**, *114*, 174–184.

(45) Liverman, M. G.; Beck, S. M.; Monts, D. L.; Smalley, R. E. Fluorescence Excitation Spectrum of the $^1A_u(n\pi) \leftarrow ^1A_g$ (0–0) Band Of Oxalyl Fluoride in a Pulsed Supersonic Free Jet. *J. Chem. Phys.* **1979**, *70*, 192–198.

(46) Ribblett, J. W.; Borst, D. R.; Pratt, D. W. Styrene and phenylacetylene: Electronic effects of conjugating substituents "off" and "on" the axis of a benzene ring. *J. Chem. Phys.* **1999**, *111*, 8454–8461.

(47) Giddings, L.; Innes, K. The Electronic Spectra and Vibrational Assignments of Carbonyl Chloride and Formyl Fluoride. *J. Mol. Spectrosc.* **1962**, *8*, 328–337.

(48) Brand, J.; Chan, W.; Liu, D.; Callomon, J.; Watson, J. The 3820 Å Band System of Propynal: Rotational Analysis of the 0-0 Band. *J. Mol. Spectrosc.* **1974**, *50*, 304–309.

(49) Gordon, R. D.; Park, W. K. The 353 nm $n\pi^\star$ Transition of 4*H*-pyran-4-one and a Deuterated Derivative. *Can. J. Chem.* **1993**, *71*, 1672–1675.

(50) Siebrand, W.; Meerts, W. L.; Pratt, D. W. Analysis and Deconvolution of Some $J' \neq 0$ Rovibronic Transitions in the High Resolution $S_1 \leftarrow S_0$ Fluorescence Excitation Spectrum of Pyrazine. *J. Chem. Phys.* **1989**, *90*, 1313–1321.

(51) Fischer, G.; Cai, Z.-L.; Reimers, J. R.; Wormell, P. Singlet and Triplet Valence Excited States of Pyrimidine. *J. Phys. Chem. A* **2003**, *107*, 3093–3106.

(52) Clouthier, D. J.; Judge, R.; Moule, D. The Laser Excitation Spectrum of Selenoformaldehyde: Vibrational Analyses of the $\mathrm{A}^1\mathrm{A}_2 \leftarrow \mathrm{X}^1\mathrm{A}_1$ and $\mathrm{a}^3\mathrm{A}_2 \leftarrow \mathrm{X}^1\mathrm{A}_1$ Electronic Transitions. *Chem. Phys.* **1987**, *114*, 417–422.

(53) Karolczak, J.; Clouthier, D. J. Pyrolysis jet spectroscopy of dichlorosilylene. *Chem. Phys. Lett.* **1993**, *201*, 409–415.

(54) Smith, T. C.; Evans, C. J.; Clouthier, D. J. Discovery of the Optically Forbidden $S_1 - S_0$ Transition of Silylidene ($H_2C{=}Si$). *J. Chem. Phys.* **2003**, *118*, 1642–1648.

(55) Harada, J.; Ogawa, K.; Tomoda, S. Molecular Motion and Conformational Interconversion of Azobenzenes in Crystals as Studied by X-ray Diffraction. *Acta Cryst. B* **1997**, *53*, 662–672.

(56) Okuyama, K.; Kakinuma, T.; Fujii, M.; Mikami, N.; Ito, M. Electronic spectra of 1,2,4,5-tetrafluorobenzene in a supersonic jet: butterfly tunneling in the excited state. *J. Phys. Chem.* **1986**, *90*, 3948–3952.

(57) Kerstel, E. R. T.; Becucci, M.; Pietraperzia, G.; Castellucci, E. Optothermal Spectroscopyof the Dissociating Lowest Electronic Singlet States of *s*-Tetrazine and Dimethyl-*s*-Tetrazine in a Molecular Beam. *J. Chem. Phys.* **1997**, *106*, 1318–1325.

(58) Judge, T. H.; Moule, D. C.; Bruno, A. E.; Steer, R. P. Thioketone Spectroscopy: An Analysis of the Lower Electronic Transitions in Thioacetone and Thioacetaldehyde. *Chem. Phys. Lett.* **1983**, *102*, 385–389.

(59) Judge, R. H.; Moule, D. C. A Vibronic Analysis of the Lower $\tilde{A}^1A$" $\leftarrow \tilde{X}^1A'$ Singlet–Singlet and $\tilde{a}^3A$" $\leftarrow \tilde{X}^1A'$ Triplet–Singlet Band Systems of Thioacrolein (2-Propenethial). *J. Chem. Phys.* **1984**, *80*, 4646–4650.

(60) Simard, B.; Hackett, P.; Steer, R. $\tilde{A} - \tilde{X}$ Laser Excitation Spectroscopy of BrClCS and $Br_2CS$ at Room Temperature and in Cold Supersonic Jets. *J. Mol. Spectrosc.* **1987**, *126*, 307–328.

(61) Subramaniam, C.; Moule, D. Analysis of the $\tilde{A}^1A$" $\leftarrow \tilde{X}^1A'$ Electronic Transition in Thiocarbonyl Chlorofluoride. *J. Mol. Spectrosc.* **1974**, *53*, 443–454.

(62) Clouthier, D.; Knight, A.; Steer, R.; Judge, R.; Moule, D. The $\tilde{B}(1A') \leftarrow \tilde{X}(1A')$ Spectrum of ClFCS. *J. Mol. Spectrosc.* **1980**, *83*, 148–160.

(63) Moule, D.; Mehra, A. The ${}^1A_2 -{}^1 A_1$ Transition in Thiocarbonyl Difluoride at 23477.1 $cm^{--1}$. *J. Mol. Spectrosc.* **1970**, *35*, 137–148.

(64) Judge, R.; Moule, D. Thiocarbonyl Spectroscopy: The $\tilde{A}^1A"\leftarrow \tilde{X}^1A'$ and $\tilde{a}^3A"\leftarrow \tilde{X}^1A'$ Electronic Transitions in Thioformyl Chloride, CHClS. *J. Mol. Struct.* **1985**, *113*, 77–84.

(65) Fujiwara, T.; Lim, E. C.; Moule, D. C. Symmetry Segregation of the Vibronic Levels Within the $S_1 \leftarrow S_0$ System of Thiophosgene, $Cl_2CS$, by Optical-Optical Double Resonance Spectroscopy. *J. Chem. Phys.* **2007**, *126*, 144304.

(66) Judge, R.; Moule, D. A Vibronic Analysis of the Lower $\tilde{A}^1A" \leftarrow \tilde{X}^1A'$ Singlet-Singlet and$\tilde{a}^3A" \leftarrow \tilde{X}^1A'$ Triplet-Singlet Band Systems of Thiopropynal. *J. Mol. Spectrosc.* **1984**, *104*, 248–252.

(67) Dyet, J.; McCoustra, M.; Pfab, J. The Visible Spectrum of Jet-Cooled $CF_3NO$. *Chem. Phys. Lett.* **1987**, *135*, 534–538.

(68) Moule, D. C.; Ng, K. H. K. The Conformational Changes Accompanying the Triplet–Singlet Electronic Excitation of Qcetaldehyde, $CH_3CHO$. *Can. J. Chem.* **1985**, *63*, 1378–1381.

(69) Hlavacek, N. C.; McAnally, M. O.; Drucker, S. Lowest Triplet $(n, \pi^\star)$ Electronic State of Acrolein: Determination of Structural Parameters by Cavity Ringdown Spectroscopy and Quantum-Chemical Methods. *J. Chem. Phys.* **2013**, *138*, 064303.

(70) Ohmori, N.; Suzuki, T.; Ito, M. Why does intersystem crossing occur in isolated molecules of benzaldehyde, acetophenone, and benzophenone? *J. Phys. Chem.* **1988**, *92*, 1086–1093.

(71) Koyanagi, M.; Kogo, Y.; Kanda, Y. Phosphorescence from the two Triplet States of *p*-Benzoquinone and Toluquinone Vapour. *Mol. Phys.* **1971**, *20*, 747–750.

(72) Tao, C.; Mukarakate, C.; Terranova, Z.; Ebben, C.; Judge, R. H.; Reid, S. A. High Resolution Study of Spin-Orbit Mixing and the Singlet-Triplet Gap in Chlorocarbene:

Stimulated Emission Pumping Spectroscopy of $CH_{35}Cl$ and $CD_{35}Cl$. *J. Chem. Phys.* **2008**, *129*, 104309.

(73) Callomon, J. H.; Davey, A. B. Rotational Analysis of the 3000 Å Absorption System of Cyanogen, $C_2N_2$. *Proc. Phys. Soc. (London)* **1963**, *82*, 335–336.

(74) Springer, M. G.; Hlavacek, N. C.; Jagusch, S. P.; Johnson, A. R.; Drucker, S. Cavity Ringdown Spectrum of the $T_1(n, \pi^\star) \rightarrow S_0$ Transition of 4-Cyclopentene-1,3-dione. *J. Phys. Chem. A* **2009**, *113*, 13318–13326, PMID: 19735120.

(75) Pillsbury, N. R.; Zwier, T. S.; Judge, R. H.; Drucker, S. Jet-Cooled Phosphorescence Excitation Spectrum of the $T_1(n, \pi^\star) \leftarrow S_0$ Transition of 2-Cyclopenten-1-one. *J. Phys. Chem. A* **2007**, *111*, 8357–8366.

(76) Ottinger, C.; Winkler, T. The Vibrational Level Structure of Trans-Glyoxal in the $T_1$ $(^3A_u)$ State. *Chem. Phys. Lett.* **1999**, *314*, 411–420.

(77) Yoshii, T.; Kiritani, M.; Hirota, N.; Baba, M. Radiative and Nonradiative Processes in the Excited States of Jet-Cooled Oxalyl Chloride. *J. Phys. Chem.* **1996**, *100*, 3354–3358.

(78) Bouvier, A.; Inard, D.; Veyret, V.; Bussery, B.; Bacis, R.; Churassy, S.; Brion, J.; Malicet, J.; Judge, R. Contribution to the Analysis of the $^3A_2 \leftarrow \tilde{X}^1A_1$ "Wulf" Transition of Ozone by High-Resolution Fourier Transform Spectrometry. *J. Mol. Spectrosc.* **1998**, *190*, 189–197.

(79) Birss, F. W.; Dong, R. Y.; Ramsay, D. A. The Band System of Propynal: Rotational Analysis of the 0–0 Band Near 4145 Å. *Can. J. Phys.* **1973**, *51*, 1810–1814.

(80) Hoffelt, L. M.; Springer, M. G.; Drucker, S. Phosphorescence Excitation Spectrum of the $T_1(n, \pi^\star) \leftarrow S_0$ Transition of 4*H*-pyran-4-one. *J. Chem. Phys.* **2008**, *128*, 104312.

(81) Ruth, A.; Fernholz, T.; Brint, R.; Mansfield, M. The $T_1 \leftarrow S_0$ Absorption Spectrum of Gaseous 4H-Pyran-4-thione. *J. Mol. Spectrosc.* **2002**, *214*, 80–86.

(82) Ottinger, C.; Vilesov, A. F. Collision-Induced Vibrational Relaxation of Pyrazine $T_1$ Observed in Spectrally Resolved Phosphorescence from a Beam. *Z. Phys. Chem.* **1995**, *188*, 111–117.

(83) Ottinger, C.; Vilesov, A.; Winkler, T. Laser-Induced Phosphorescence of Jet-Cooled Pyrimidine. *Chem. Phys. Lett.* **1993**, *208*, 299–306.

(84) Judge, R. H.; Clouthier, D. J.; Moule, D. C. The Laser Excitation Spectrum of $CH_2Se$ and $CD_2Se$ in the Near Infrared. *J. Chem. Phys.* **1988**, *89*, 1807–1812.

(85) Karolczak, J.; Judge, R. H.; Clouthier, D. J. Experimental Determination of the Structure of $SiF_2$ in Its Excited Triplet State. *J. Am. Chem. Soc.* **1995**, *117*, 9523–9528.

(86) Huang, C.-L.; Ju, S.-S.; Chen, I.-C.; Merer, A. J.; Ni, C.-K.; Kung, A. High-Resolution Spectroscopy of Jet-Cooled $^{32}SO_2$ and $^{34}SO_2$: The $\tilde{a}^3B_1 - -\tilde{X}^1A_1$, $2_0^1$ and $1_0^1$ Bands. *J. Mol. Spectrosc.* **2000**, *203*, 151 –157.

(87) Livak, D.; Innes, K. A Triplet-Singlet Transition of *s*-Tetrazine. *J. Mol. Spectrosc.* **1971**, *39*, 115–122.

(88) Judge, R. H.; Moule, D. C.; Bruno, A. E.; Steer, R. P. Thiocarbonyl Spectroscopy: Methyl Torsional Vibrations and Internal Rotational Barriers of Thioacetaldehyde in its $\tilde{a}^3A''$ and $\tilde{X}^1A'$ States. *J. Chem. Phys.* **1987**, *87*, 60–67.

(89) Moule, D. C.; Smeyers, Y. G.; Senent, M. L.; Clouthier, D. J.; Karolczak, J.; Judge, R. H. An Analysis of the Methyl Rotation Dynamics in the $S_0(\tilde{X}^1A_1)$ and $T_1(\tilde{a}^3A_2)$ States of Thioacetone, $(CH_3)_2CS$ and $(CD_3)_2CS$ from Pyrolysis Jet Spectra. *J. Chem. Phys.* **1991**, *95*, 3137–3146.

(90) Fujiwara, T.; Lim, E. C.; Judge, R. H.; Moule, D. C. An Optical-Optical Double Resonance Probe of the Lowest Triplet State of Jet-Cooled Thiophosgene: Rovibronic Structures and Electronic Relaxation. *J. Chem. Phys.* **2006**, *124*, 124301.

(91) Ohta, N.; Fujita, M.; Takemura, T.; Shindo, Y.; Baba, H. Phosphorescence of *s*-Triazine Vapor. *Chem. Phys. Lett.* **1983**, *97*, 81–84.
